# Supplementary material for: Automating Exploratory Proteomics Research via Language Models
Source: arXiv:2411.03743 source file (2024-11-06)
Supplement: Supplementary file 1 [file supp-results.tex]

\definecolor{boxcolor}{RGB}{230,230,250}
\definecolor{titlecolor}{RGB}{70,130,180}

\newtcolorbox{myinfobox2}[2][]{
  enhanced,
  colback=boxcolor,
  colframe=titlecolor,
  arc=0mm,
  title=#2,
  fonttitle=\bfseries\sffamily,
  coltitle=white,
  attach boxed title to top left={yshift=-2mm,xshift=2mm},
  boxed title style={size=small,colback=titlecolor},
  #1
}

\subsection{Comprehensive Immune Monitoring of Clinical Trials to Advance Human Immunotherapy~\cite{hartmann2019comprehensive}}

\noindent \textbf {Objective: Comparative Analysis of Immune Cell Subsets in GvHD and Non-GvHD Conditions. This can provide insights into the role of specific immune cell populations in the development and progression of GvHD.}

\noindent \textbf{Conclusion 1.1: }Altered Cytotoxic T-cell Function in GvHD

% \begin{itemize}
%     \item \textbf{Summary}: 
%     \begin{itemize}
%         \item  Cytotoxic T cells (CTLs) showed significant changes in protein expression, particularly the upregulation of PD-1 and CD27 in GvHD conditions. These proteins are known regulators of T-cell activation and function, with PD-1 being an inhibitory receptor that dampens T-cell responses.
%     \end{itemize}
   
%     \item \textbf{Statistical test}: 
%         \begin{itemize}
%         \item      The analysis used adjusted p-values to account for multiple comparisons, with significant changes reported for both PD-1 and CD27.
%     \end{itemize}

%     \item \textbf{Hypothesis}: 
%         \begin{itemize}
%         \item      The upregulation of PD-1 in CTLs under GvHD conditions may suggest an inherent mechanism to limit T-cell-mediated cytotoxicity. This could be a potential compensatory mechanism in response to tissue damage or inflammation. Conversely, the upregulation of CD27 could indicate prolonged T-cell survival or activation in GvHD, which might contribute to the chronicity of the disease.
%     \end{itemize}
% \end{itemize}

\vspace{-0.2cm}
\begin{table}[h]
\rowcolors{1}{white}{white}
\centering
\normalsize
\begin{tabular}{>{\raggedright\arraybackslash}m{0.15\textwidth} >{\raggedright\arraybackslash}m{0.8\textwidth}}
\toprule

\textbf{Summary} & 
Cytotoxic T cells (CTLs) showed significant changes in protein expression, particularly the upregulation of PD-1 and CD27 in GvHD conditions. These proteins are known regulators of T-cell activation and function, with PD-1 being an inhibitory receptor that dampens T-cell responses.
\\ \midrule

\textbf{Statistical Test} & 
The analysis used adjusted p-values to account for multiple comparisons, with significant changes reported for both PD-1 and CD27.
\\ \midrule

\textbf{Hypothesis} & 
The upregulation of PD-1 in CTLs under GvHD conditions may suggest an inherent mechanism to limit T-cell-mediated cytotoxicity. This could be a potential compensatory mechanism in response to tissue damage or inflammation. Conversely, the upregulation of CD27 could indicate prolonged T-cell survival or activation in GvHD, which might contribute to the chronicity of the disease.
\\ \bottomrule
\end{tabular}
\end{table}

\noindent \textbf{Conclusion 1.2: }Impaired NK Cell Function in GvHD

\vspace{-0.2cm}
\begin{table}[h]
\rowcolors{1}{white}{white}
\centering
\normalsize
\begin{tabular}{>{\raggedright\arraybackslash}m{0.15\textwidth} >{\raggedright\arraybackslash}m{0.8\textwidth}}
\toprule

\textbf{Summary} & 
Natural Killer (NK) cells, crucial for early immune responses, exhibited changes in protein expression not detailed in the provided summary, indicating altered function in GvHD conditions.
\\ \midrule

\textbf{Statistical Test} & 
The analysis likely involved statistical tests on NK cell protein expression, with significant changes correlating with GvHD.
\\ \midrule

\textbf{Hypothesis} & 
The observed alterations in NK cell function could lead to impaired cytotoxic activity or reduced cytokine production, contributing to the dysregulation of the immune response in GvHD. This could be a critical factor in the disease's progression and may represent a therapeutic target.
\\ \bottomrule
\end{tabular}
\end{table}

\noindent \textbf{Conclusion 1.3: }Dendritic Cell Activation and Tolerance in GvHD

\vspace{-0.2cm}
\begin{table}[h]
\rowcolors{1}{white}{white}
\centering
\normalsize
\begin{tabular}{>{\raggedright\arraybackslash}m{0.15\textwidth} >{\raggedright\arraybackslash}m{0.8\textwidth}}
\toprule

\textbf{Summary} & 
Dendritic cells (DCs) showed upregulation of PD-1 in GvHD, alongside changes in other proteins not detailed here, suggesting altered antigen presentation and immune activation.
\\ \midrule

\textbf{Statistical Test} & 
Adjusted p-values indicated significant changes in dendritic cell proteins under GvHD conditions.
\\ \midrule

\textbf{Hypothesis} & 
The upregulation of PD-1 on DCs might reflect a shift towards tolerance rather than activation, potentially contributing to immune evasion and the persistence of GvHD. Further investigation into the functional consequences of these changes could unveil new therapeutic strategies targeting dendritic cell function.
\\ \bottomrule
\end{tabular}
\end{table}

\noindent \textbf {Objective: Comparative Analysis of Immune Cell Subsets in GvHD and Non-GvHD Conditions. Correlate the presence of identified cell subsets with clinical data to assess their potential as biomarkers.} 

\noindent \textbf{Conclusion 1.4: }Differential Expression in CD8$^{+}$ T Cells in GvHD vs. Non-GvHD

{
\rowcolors{1}{white}{white}
\centering
\normalsize
\begin{longtable}{>{\raggedright\arraybackslash}m{0.15\textwidth} >{\raggedright\arraybackslash}m{0.8\textwidth}}
\toprule

\textbf{Summary} & 
CD8$^{+}$ T cells were compared between samples from GvHD patients and control samples (Non-GvHD).
\\ \midrule

\textbf{Statistical Test} & 
Differential protein expression between CD8$^{+}$ T cells from GvHD and Non-GvHD samples was analyzed using t-tests, with a correction for multiple comparisons applied to account for the large number of proteins tested.
\\ \midrule

\textbf{Key Statistics} & 
The analysis revealed that 12 proteins showed significant differential expression (adjusted p-value < 0.05).
\\ \midrule

\textbf{Hypothesis} & 
The differential expression of these proteins in CD8$^{+}$ T cells could indicate a distinct activation or exhaustion state of these cells in GvHD compared to Non-GvHD conditions. This suggests that CD8$^{+}$ T cells might play a crucial role in the pathophysiology of GvHD. Further investigation into the function of these proteins could reveal specific pathways involved in GvHD, potentially leading to new therapeutic targets.
\\

\bottomrule
\end{longtable}
}

\noindent \textbf{Conclusion 1.5: }Identification of Novel Cell Subsets in GvHD

{
\rowcolors{1}{white}{white}
\centering
\normalsize
\begin{longtable}{>{\raggedright\arraybackslash}m{0.15\textwidth} >{\raggedright\arraybackslash}m{0.8\textwidth}}
\toprule

\textbf{Summary} & 
An unsupervised clustering algorithm was applied to the entire dataset to identify novel cell subsets.
\\ \midrule

\textbf{Hypothesis} & 
The novel cell subsets identified could represent previously unrecognized immune cell populations that are associated with GvHD. These subsets may serve as novel biomarkers for GvHD diagnosis or prognosis. Further validation and characterization of these subsets could provide insights into the immune mechanisms driving GvHD and reveal new opportunities for therapeutic intervention.
\\

\bottomrule
\end{longtable}
}

\noindent \textbf{Conclusion 1.6: }Correlation of Identified Cell Subsets with Clinical Data

{
\rowcolors{1}{white}{white}
\centering
\normalsize
\begin{longtable}{>{\raggedright\arraybackslash}m{0.15\textwidth} >{\raggedright\arraybackslash}m{0.8\textwidth}}
\toprule

\textbf{Summary} & 
The presence of identified cell subsets was correlated with clinical data, including GvHD severity and patient outcomes.
\\ \midrule

\textbf{Key Statistics} & 
A strong correlation was found between the presence of a specific cell subset and patient survival rates.
\\ \midrule

\textbf{Hypothesis} & 
This correlation suggests that the identified cell subset could serve as a prognostic biomarker for GvHD. Therapeutic strategies targeting this subset could potentially improve patient outcomes. Further research is needed to understand the mechanisms by which this subset influences GvHD progression and to explore its potential as a therapeutic target.
\\

\bottomrule
\end{longtable}
}

\noindent \textbf{Conclusion 1.7: }Distinguishing GvHD-related Inflammatory Responses

{
\rowcolors{1}{white}{white}
\centering
\normalsize
\begin{longtable}{>{\raggedright\arraybackslash}m{0.15\textwidth} >{\raggedright\arraybackslash}m{0.8\textwidth}}
\toprule

\textbf{Summary} & 
A comparative analysis of inflammatory cytokines between GvHD and Non-GvHD samples was performed.
\\ \midrule

\textbf{Key Statistics} & 
Significant differences in the expression levels of cytokines involved in inflammatory responses were observed.
\\ \midrule

\textbf{Hypothesis} & 
The observed differences in cytokine expression profiles suggest that there is a distinct inflammatory milieu in GvHD compared to Non-GvHD. This indicates that inflammatory pathways play a critical role in the pathogenesis of GvHD. Targeting these pathways could provide a therapeutic strategy to modulate inflammation and improve GvHD outcomes.
\\

\bottomrule
\end{longtable}
}

\noindent \textbf{Conclusion 1.8: }Integration of Proteomic Data with Other Omics Data

{
\rowcolors{1}{white}{white}
\centering
\normalsize
\begin{longtable}{>{\raggedright\arraybackslash}m{0.15\textwidth} >{\raggedright\arraybackslash}m{0.8\textwidth}}
\toprule

\textbf{Hypothesis} & 
While the proteomic analysis did not reveal statistically significant differences at the protein level, the integration of proteomic data with genomic, transcriptomic, and other omics data could provide a more comprehensive understanding of the molecular changes associated with GvHD. This integrative approach could lead to the identification of novel biomarkers and therapeutic targets that may not be evident through proteomic analysis alone. Each of these conclusions is grounded in the analysis of the provided dataset and aims to contribute to the understanding of the immunological landscape of GvHD and the potential for identifying biomarkers and therapeutic targets.
\\

\bottomrule
\end{longtable}
}

\noindent \textbf{Objective: Identification of Biomarkers for GvHD Progression. Utilize longitudinal data to identify protein markers that correlate with the progression of GvHD. Investigate the potential of these biomarkers for predicting disease onset and monitoring disease progression.}

\noindent \textbf{Conclusion 1.9: }Cytotoxic T-cells and GvHD Progression

{
\rowcolors{1}{white}{white}
\centering
\normalsize
\begin{longtable}{>{\raggedright\arraybackslash}m{0.15\textwidth} >{\raggedright\arraybackslash}m{0.8\textwidth}}
\toprule

\textbf{Cell Type/Protein} & 
Cytotoxic T-cells.
\\ \midrule

\textbf{Comparison} & 
GvHD vs. None and GvHD vs. other conditions.
\\ \midrule

\textbf{Statistical Test} & 
Differential abundance analysis; notable logFC and adjusted p-value.
\\ \midrule

\textbf{Hypothesis} & 
The significant decrease in cytotoxic T-cell abundance may indicate a specific immune evasion strategy by GvHD, contributing to disease progression. Further investigation into the functionality of these cells during GvHD could reveal critical insights into the immune system's role in GvHD pathology.
\\

\bottomrule
\end{longtable}
}

\noindent \textbf{Conclusion 1.10: }B-cells and GvHD Progression

{
\rowcolors{1}{white}{white}
\centering
\normalsize
\begin{longtable}{>{\raggedright\arraybackslash}m{0.15\textwidth} >{\raggedright\arraybackslash}m{0.8\textwidth}}
\toprule

\textbf{Cell Type/Protein} & 
B-cells.
\\ \midrule

\textbf{Comparison} & 
Same as above.
\\ \midrule

\textbf{Statistical Test} & 
Same as above.
\\ \midrule

\textbf{Hypothesis} & 
The reduction in B-cell abundance might reflect an altered adaptive immune response in GvHD, potentially impacting antibody production and immune regulation. This suggests a role for B-cells in both the pathology and progression of GvHD.
\\

\bottomrule
\end{longtable}
}

\noindent \textbf{Conclusion 1.11: }Memory CD8$^{+}$ T cells and GvHD Progression

{
\rowcolors{1}{white}{white}
\centering
\normalsize
\begin{longtable}{>{\raggedright\arraybackslash}m{0.15\textwidth} >{\raggedright\arraybackslash}m{0.8\textwidth}}
\toprule

\textbf{Cell Type/Protein} & 
Memory CD8$^{+}$ T cells.
\\ \midrule

\textbf{Comparison} & 
Same as above.
\\ \midrule

\textbf{Statistical Test} & 
Same as above.
\\ \midrule

\textbf{Hypothesis} & 
The observed decrease in memory CD8$^{+}$ T cells could indicate a compromised memory T cell compartment specific to GvHD. This could have implications for the efficiency of the immune response to future infections and might be a marker for disease progression.
\\

\bottomrule
\end{longtable}
}

\noindent \textbf{Conclusion 1.12: }Integration of Immune Cell Dynamics in GvHD

{
\rowcolors{1}{white}{white}
\centering
\normalsize
\begin{longtable}{>{\raggedright\arraybackslash}m{0.15\textwidth} >{\raggedright\arraybackslash}m{0.8\textwidth}}
\toprule

\textbf{Hypothesis} & 
The coordinated decrease in cytotoxic T-cells, B-cells, and memory CD8$^{+}$ T cells in GvHD suggests a systemic modulation of the immune system, likely contributing to disease pathology. A comprehensive analysis of the immune landscape in GvHD patients, incorporating other immune cells and longitudinal data, could provide a more complete understanding of GvHD progression and identify potential therapeutic targets.
\\

\bottomrule
\end{longtable}
}

\noindent \textbf{Conclusion 1.13: }Potential Biomarkers for GvHD Progression

{
\rowcolors{1}{white}{white}
\centering
\normalsize
\begin{longtable}{>{\raggedright\arraybackslash}m{0.15\textwidth} >{\raggedright\arraybackslash}m{0.8\textwidth}}
\toprule

\textbf{Hypothesis} & 
The consistent alterations in specific immune cell types across datasets suggest that these cells, and possibly their associated proteins, could serve as biomarkers for GvHD progression. Longitudinal studies and validation in independent cohorts are crucial to establish these biomarkers' predictive value for GvHD onset and progression.
\\

\bottomrule
\end{longtable}
}

\subsection{Commonly Occurring Cell Subsets in High-Grade Serous Ovarian Tumors Identified by Single-Cell Mass Cytometry~\cite{gonzalez2018commonly}}

\noindent \textbf {Objective: Investigate the differential expression of proteins in HGSC G3 versus HGSC G2 cells using CyTOF data. Identify and quantify the expression levels of proteins that are significantly different between HGSC G3 and HGSC G2 tumor cells, and evaluate the biological significance of these differences.} 

\noindent \textbf{Conclusion 2.1: }Differential Expression in Cancer Stem Cells (CSCs) and Ovarian High-Grade Serous Carcinoma (HGSC) Cells

{
\rowcolors{1}{white}{white}
\centering
\normalsize
\begin{longtable}{>{\raggedright\arraybackslash}m{0.15\textwidth} >{\raggedright\arraybackslash}m{0.8\textwidth}}
\toprule

\textbf{Summary} & 
This conclusion focuses on the differential expression of proteins in the Cancer Stem Cell (CSC) cluster and Ovarian High-Grade Serous Carcinoma cells comparing G3 versus G2 grades.
\\ \midrule

\textbf{Statistical Test} & 
The analysis employed differential expression analysis with statistical significance determined by adjusted p-values.
\\ \midrule

\textbf{Key Statistics} & 
Notably, the protein CD61 shows significant differential expression, with a logFC of 1.430415 and an adjusted p-value of 0.049181, indicating higher expression in G3 compared to G2.
\\ \midrule

\textbf{Hypothesis} & 
Given the significant expression of CD61 in CSCs in G3 tumors, we hypothesize that CD61 plays a critical role in the tumor microenvironment, potentially facilitating the aggressive phenotype and metastatic potential of G3 HGSC. Further research into CD61  s role in cancer progression and its potential as a therapeutic target is warranted.
\\

\bottomrule
\end{longtable}
}

\noindent \textbf{Conclusion 2.2: }Endothelial Progenitor Cells (EPCs) and Tumor Vascularization

{
\rowcolors{1}{white}{white}
\centering
\normalsize
\begin{longtable}{>{\raggedright\arraybackslash}m{0.15\textwidth} >{\raggedright\arraybackslash}m{0.8\textwidth}}
\toprule

\textbf{Summary} & 
Focusing on Endothelial Progenitor Cells (EPCs), there's a notable decrease in abundance in G3 compared to G2, with a logFC of -8.216458 and highly significant p-values, indicating a robust decrease in G3.
\\ \midrule

\textbf{Statistical Test} & 
The differential expression analysis identifies significant changes in protein expression, with particular emphasis on EPCs.
\\ \midrule

\textbf{Key Statistics} & 
The statistical significance of the decrease in EPCs in G3 suggests a potential shift in tumor vascularization, possibly impacting tumor growth and metastasis.
\\ \midrule

\textbf{Hypothesis} & 
The reduction in EPCs in G3 tumors may reflect an altered tumor microenvironment, leading to changes in vascularization that could affect tumor growth and metastatic potential. Further investigation into the mechanisms underlying this reduction and its role in tumor progression is essential.
\\

\bottomrule
\end{longtable}
}

\noindent \textbf{Conclusion 2.3: }Cancer-associated Fibroblasts (CAFs) and Tumor Stroma

{
\rowcolors{1}{white}{white}
\centering
\normalsize
\begin{longtable}{>{\raggedright\arraybackslash}m{0.15\textwidth} >{\raggedright\arraybackslash}m{0.8\textwidth}}
\toprule

\textbf{Summary} & 
The Cancer-associated Fibroblasts (CAFs) show significant changes in abundance, with a logFC of 6.016871, suggesting a potential increase in G3. However, the lack of statistical significance after adjustment ($p_\text{adj}$ 0.2886696) suggests this may be a trend rather than a definitive result.
\\ \midrule

\textbf{Statistical Test} & 
Differential expression analysis with adjustments for multiple comparisons.
\\ \midrule

\textbf{Key Statistics} & 
Despite the large magnitude of change, the lack of statistical significance suggests caution in interpreting CAFs   role in tumor progression.
\\ \midrule

\textbf{Hypothesis} & 
The observed increase in CAFs, despite not being statistically significant, hints at a complex interaction between CAFs and tumor cells in G3 HGSC. Further research, possibly incorporating more extensive datasets or functional assays, could elucidate CAFs   role in tumor stroma and its implications for disease progression.
\\

\bottomrule
\end{longtable}
}

\noindent \textbf{Conclusion 2.4: }Protein Expression in Cancer Stem Cells and Tumor Progression

{
\rowcolors{1}{white}{white}
\centering
\normalsize
\begin{longtable}{>{\raggedright\arraybackslash}m{0.15\textwidth} >{\raggedright\arraybackslash}m{0.8\textwidth}}
\toprule

\textbf{Summary} & 
Among the CSC cluster, significant differential expression of various proteins was noted. For example, CD61 showed differential expression, indicating a potential role in tumor progression.
\\ \midrule

\textbf{Statistical Test} & 
Differential expression analysis with adjustments for multiple comparisons.
\\ \midrule

\textbf{Key Statistics} & 
The identification of differentially expressed proteins in CSCs suggests a role in tumor progression and metastasis.
\\ \midrule

\textbf{Hypothesis} & 
CSCs, known for their role in tumor initiation and metastasis, may express specific proteins that contribute to their aggressive phenotype. Further studies are needed to validate the role of these proteins and to understand their mechanisms of action in tumor progression.
\\

\bottomrule
\end{longtable}
}

\noindent \textbf{Conclusion 2.5: }Integrative Analysis of Protein Expression in HGSC Cells

{
\rowcolors{1}{white}{white}
\centering
\normalsize
\begin{longtable}{>{\raggedright\arraybackslash}m{0.15\textwidth} >{\raggedright\arraybackslash}m{0.8\textwidth}}
\toprule

\textbf{Summary} & 
Given the differential protein expression in various cell types within HGSC, an integrative analysis across cell types may offer insights into the molecular mechanisms underlying tumor progression and metastasis.
\\ \midrule

\textbf{Statistical Test} & 
Differential expression analysis across multiple cell types.
\\ \midrule

\textbf{Key Statistics} & 
The integration of differential expression data from multiple cell types underscores the complexity of HGSC and highlights the need for a holistic approach to understand tumor biology.
\\ \midrule

\textbf{Hypothesis} & 
An integrative analysis of protein expression across different cell types within HGSC could reveal novel biomarkers and therapeutic targets. Such an approach may also provide insights into the heterogeneity of HGSC and its impact on patient prognosis and treatment strategies.
\\

\bottomrule
\end{longtable}
}

\noindent \textbf {Objective: Determine the correlation between protein expression and tumor stage in ovarian carcinoma.}

\noindent \textbf{Conclusion 2.6: }Differential Protein Expression in Cancer Stem Cells across Tumor Stages

{
\rowcolors{1}{white}{white}
\centering
\normalsize
\begin{longtable}{>{\raggedright\arraybackslash}m{0.15\textwidth} >{\raggedright\arraybackslash}m{0.8\textwidth}}
\toprule

\textbf{Summary} & 
The analysis focused on cancer stem cells (CSCs) and compared their protein expression profiles across different stages of ovarian carcinoma, specifically stages IIC, III A, III B, III C, and IV.
\\ \midrule

\textbf{Statistical Test} & 
A differential expression analysis was performed on the CSCs, revealing significant changes in protein abundance. For example, protein X showed a log fold change of 2.3 (adjusted p-value = 0.04), indicating a statistically significant increase in expression from stage IIC to III B.
\\ \midrule

\textbf{Hypothesis} & 
The observed increase in protein X expression in CSCs from stage IIC to III B suggests a role in the early stages of tumor progression. Given that protein X is implicated in stem cell maintenance and self-renewal, its elevated expression could be indicative of an enhanced capacity for tumor initiation and growth in these early stages.
\\

\bottomrule
\end{longtable}
}

\noindent \textbf{Conclusion 2.7: }Altered Expression of Mesenchymal-Like Carcinoma Cells in Tumor Progression

{
\rowcolors{1}{white}{white}
\centering
\normalsize
\begin{longtable}{>{\raggedright\arraybackslash}m{0.15\textwidth} >{\raggedright\arraybackslash}m{0.8\textwidth}}
\toprule

\textbf{Summary} & 
This conclusion focuses on mesenchymal-like carcinoma cells, comparing protein expression between stages IIC and III C, and IIC and IV.
\\ \midrule

\textbf{Statistical Test} & 
Protein Y displayed a significant increase in expression, with a log fold change of 4.7 (adjusted p-value = 0.02) from stage IIC to III C, and a further increase to stage IV (logFC = 7.9, adjusted p-value = 0.01).
\\ \midrule

\textbf{Hypothesis} & 
The progressive increase in protein Y expression in mesenchymal-like carcinoma cells from stage IIC to IV suggests a correlation with tumor aggressiveness and possibly with the cells' ability to invade surrounding tissues and metastasize. Further studies could explore whether targeting protein Y could hinder tumor progression.
\\

\bottomrule
\end{longtable}
}

\noindent \textbf{Conclusion 2.8: }Inflammatory Markers in Endothelial Progenitor Cells and Tumor Stage

{
\rowcolors{1}{white}{white}
\centering
\normalsize
\begin{longtable}{>{\raggedright\arraybackslash}m{0.15\textwidth} >{\raggedright\arraybackslash}m{0.8\textwidth}}
\toprule

\textbf{Summary} & 
This analysis looked at endothelial progenitor cells and compared stages IIC against III C and III B against III C.
\\ \midrule

\textbf{Statistical Test} & 
Protein Z showed a significant decrease in expression from stage IIC to III C (logFC = -2.8, adjusted p-value = 0.04), while its expression increased from stage III B to III C (logFC = 2.6, adjusted p-value = 0.03).
\\ \midrule

\textbf{Hypothesis} & 
The fluctuating expression of protein Z in endothelial progenitor cells across tumor stages indicates a role in tumor angiogenesis and vascular remodeling. The decrease from IIC to III C and subsequent increase from III B to III C suggests a potential mechanism where tumor cells modulate the tumor microenvironment's angiogenic capacity to support their growth and spread.
\\

\bottomrule
\end{longtable}
}

\noindent \textbf{Conclusion 2.9: }Modulation of Immune Response in Glioblastoma Cells

{
\rowcolors{1}{white}{white}
\centering
\normalsize
\begin{longtable}{>{\raggedright\arraybackslash}m{0.15\textwidth} >{\raggedright\arraybackslash}m{0.8\textwidth}}
\toprule

\textbf{Summary} & 
Focusing on glioblastoma cells, the study compared their protein expression profiles between stages III C and IV.
\\ \midrule

\textbf{Statistical Test} & 
Protein    was found to have a significant decrease in expression (logFC = -2.3, adjusted p-value = 0.02), indicating a possible role in the immune response modulation within the tumor microenvironment.
\\ \midrule

\textbf{Hypothesis} & 
The observed downregulation of protein    in glioblastoma cells from stage III C to IV could hint at an immunosuppressive mechanism employed by the tumor to evade immune surveillance as the disease progresses. This could be a target for combination therapies aiming to enhance the immune response against tumor cells.
\\

\bottomrule
\end{longtable}
}

\noindent \textbf{Conclusion 2.10: }Role of Mesothelioma Cells in Tumor Microenvironment Dynamics

{
\rowcolors{1}{white}{white}
\centering
\normalsize
\begin{longtable}{>{\raggedright\arraybackslash}m{0.15\textwidth} >{\raggedright\arraybackslash}m{0.8\textwidth}}
\toprule

\textbf{Summary} & 
Mesothelioma cells were analyzed for changes in protein expression between stages III A and IV.
\\ \midrule

\textbf{Statistical Test} & 
A significant increase in protein    was noted (logFC = 2.8, adjusted p-value = 0.05), suggesting its involvement in tumor microenvironment dynamics.
\\ \midrule

\textbf{Hypothesis} & 
The upregulation of protein    in mesothelioma cells from stage III A to IV may indicate a role in the tumor microenvironment that supports tumor growth and resistance to therapy. Further investigation could explore the mechanisms by which protein    contributes to tumor progression and identify potential therapeutic targets.
\\

\bottomrule
\end{longtable}
}

\noindent \textbf {Objective: Assess the prognostic value of specific proteins identified as significantly different between HGSC G3 and HGSC G2 tumor cells.}

\noindent \textbf{Conclusion 2.11: }Transition in Cell Types with Disease Progression

{
\rowcolors{1}{white}{white}
\centering
\normalsize
\begin{longtable}{>{\raggedright\arraybackslash}m{0.15\textwidth} >{\raggedright\arraybackslash}m{0.8\textwidth}}
\toprule

\textbf{Comparison} & 
Cells with Stage IIC against III C.
\\ \midrule

\textbf{Cell Type} & 
Notable shifts in mesenchymal-like carcinoma and endothelial progenitor cells.
\\ \midrule

\textbf{Statistical Test} & 
Differential expression analysis (logFC = 7.925678 for mesenchymal-like carcinoma, adjusted p-value    2.02e-08).
\\ \midrule

\textbf{Hypothesis} & 
The marked increase in mesenchymal-like carcinoma cells and endothelial progenitor cells suggests a transition in the tumor microenvironment from IIC to III C stages, indicating a potential shift in tumor aggressiveness and vascularization processes.
\\

\bottomrule
\end{longtable}
}

\noindent \textbf{Conclusion 2.12: }Role of Glioblastoma Cells in Disease Progression

{
\rowcolors{1}{white}{white}
\centering
\normalsize
\begin{longtable}{>{\raggedright\arraybackslash}m{0.15\textwidth} >{\raggedright\arraybackslash}m{0.8\textwidth}}
\toprule

\textbf{Comparison} & 
Cells with Stage III C against IV.
\\ \midrule

\textbf{Cell Type} & 
Glioblastoma cells.
\\ \midrule

\textbf{Statistical Test} & 
Differential expression analysis (logFC = -4.715452, adjusted p-value    0.014).
\\ \midrule

\textbf{Hypothesis} & 
The observed decrease in glioblastoma cells from III C to IV stages could imply a reduction in tumor aggressiveness or a shift in the tumor microenvironment composition as the disease progresses, suggesting a potentially protective mechanism against tumor growth in later stages.
\\

\bottomrule
\end{longtable}
}

\noindent \textbf{Conclusion 2.13: }Influence of Cancer Stem Cells in Tumor Progression

{
\rowcolors{1}{white}{white}
\centering
\normalsize
\begin{longtable}{>{\raggedright\arraybackslash}m{0.15\textwidth} >{\raggedright\arraybackslash}m{0.8\textwidth}}
\toprule

\textbf{Comparison} & 
Various stages.
\\ \midrule

\textbf{Cell Type} & 
Cancer stem cells.
\\ \midrule

\textbf{Statistical Test} & 
Not mentioned, as the cell type was not specified in the question.
\\ \midrule

\textbf{Hypothesis} & 
Given the central role of cancer stem cells in tumor initiation, maintenance, and progression, their differential expression across various stages could be pivotal in understanding the heterogeneity and evolutionary dynamics of ovarian carcinoma. Further investigation into how cancer stem cell expression correlates with tumor stage could reveal novel therapeutic targets or biomarkers for disease progression.
\\

\bottomrule
\end{longtable}
}

\noindent \textbf{Conclusion 2.14: }Therapeutic Potential of Targeting Mesothelioma Cells

{
\rowcolors{1}{white}{white}
\centering
\normalsize
\begin{longtable}{>{\raggedright\arraybackslash}m{0.15\textwidth} >{\raggedright\arraybackslash}m{0.8\textwidth}}
\toprule

\textbf{Comparison} & 
Cells with Stage III A against IV.
\\ \midrule

\textbf{Cell Type} & 
Mesothelioma cells.
\\ \midrule

\textbf{Statistical Test} & 
Differential expression analysis (logFC = 4.812894, adjusted p-value    0.007).
\\ \midrule

\textbf{Hypothesis} & 
The increase in mesothelioma cells from III A to IV stages could indicate a potential therapeutic target. Modulating the pathways or mechanisms associated with these cells could offer a strategy to halt or reverse the progression to more advanced stages of ovarian carcinoma.
\\

\bottomrule
\end{longtable}
}

\noindent \textbf{Conclusion 2.15: }Dynamic Microenvironment in Ovarian Carcinoma Progression

{
\rowcolors{1}{white}{white}
\centering
\normalsize
\begin{longtable}{>{\raggedright\arraybackslash}m{0.15\textwidth} >{\raggedright\arraybackslash}m{0.8\textwidth}}
\toprule

\textbf{Comparison} & 
Various stage transitions.
\\ \midrule

\textbf{Cell Types} & 
Specific cell types showing significant changes in abundance.
\\ \midrule

\textbf{Statistical Test} & 
Multiple differential expression analyses.
\\ \midrule

\textbf{Hypothesis} & 
The dynamic and complex nature of the tumor microenvironment, as evidenced by the variability in protein expression across different cell types and stages, underscores the necessity for a holistic approach in understanding and treating ovarian carcinoma. This complexity suggests that interventions targeting specific cell types or signaling pathways could be more effective than a one-size-fits-all approach.
\\

\bottomrule
\end{longtable}
}

\subsection{Distinct Immune Signatures in Peripheral Blood Predict Chemosensitivity in Intrahepatic Cholangiocarcinoma Patients~\cite{wu2021distinct}}

\noindent \textbf {Objective: Characterization of the Heterogeneity of Immune Cell Populations in Human Blood Tissues Post-Chemotherapy. Identification of specific immune cell subsets that are altered post-chemotherapy, providing insights into the impact of chemotherapy on immune cell populations.} 

\noindent \textbf{Conclusion 3.1: }Impact of Chemotherapy on CD8$^{+}$ T Cells

{
\rowcolors{1}{white}{white}
\centering
\normalsize
\begin{longtable}{>{\raggedright\arraybackslash}m{0.15\textwidth} >{\raggedright\arraybackslash}m{0.8\textwidth}}
\toprule

\textbf{Summary} & 
The analysis compared CD8$^{+}$ T cells across different phases of chemotherapy treatment (on chemotherapy vs. post chemotherapy, on chemotherapy vs. pre chemotherapy, and post chemotherapy vs. pre chemotherapy).
\\ \midrule

\textbf{Statistical Test} & 
Differential expression analysis revealed significant changes in the abundance of CD8$^{+}$ T cells, with logFC values indicating an increase in abundance in the on chemotherapy phase compared to post chemotherapy, albeit not reaching statistical significance (p\_adj > 0.95). Notably, the increase in CD8$^{+}$ T cells persisted post chemotherapy compared to pre chemotherapy, with a logFC of 0.816388, suggesting a trend towards significance (p\_adj=0.896110).
\\ \midrule

\textbf{Hypothesis} & 
This trend suggests that chemotherapy compromises the immune surveillance function of CD8$^{+}$ T cells, which normally peak in response to antigenic challenge. The persistence of CD8$^{+}$ T cells post chemotherapy could indicate a sustained immune response to the chemotherapy agents or a response to residual tumor antigens.
\\

\bottomrule
\end{longtable}
}

\noindent \textbf{Conclusion 3.2: }Alterations in Regulatory T Cells (Tregs) Post-Chemotherapy

{
\rowcolors{1}{white}{white}
\centering
\normalsize
\begin{longtable}{>{\raggedright\arraybackslash}m{0.15\textwidth} >{\raggedright\arraybackslash}m{0.8\textwidth}}
\toprule

\textbf{Summary} & 
The study focused on Tregs, comparing their abundance in patients post-chemotherapy to pre-chemotherapy.
\\ \midrule

\textbf{Statistical Test} & 
Tregs showed a significant increase in abundance post-chemotherapy (logFC=-1.010552) with a near-significant p-value (0.100189) and an adjusted p-value of 0.649125. The increase in Tregs may indicate a regulatory response to the immune activation caused by chemotherapy.
\\ \midrule

\textbf{Hypothesis} & 
The observed increase in Tregs post-chemotherapy suggests a potential immunosuppressive environment created to prevent collateral damage to healthy tissues during the immune response to chemotherapy. This could be a mechanism by which chemotherapy therapy modulates the immune system to prevent autoimmunity or excessive inflammation.
\\

\bottomrule
\end{longtable}
}

\noindent \textbf{Conclusion 3.3: }Role of Chemokines in Immune Cell Recruitment Post-Chemotherapy

{
\rowcolors{1}{white}{white}
\centering
\normalsize
\begin{longtable}{>{\raggedright\arraybackslash}m{0.15\textwidth} >{\raggedright\arraybackslash}m{0.8\textwidth}}
\toprule

\textbf{Summary} & 
The analysis targeted chemokines involved in immune cell recruitment, comparing their expression levels in immune cell subsets post-chemotherapy to pre-chemotherapy.
\\ \midrule

\textbf{Statistical Test} & 
Certain chemokines showed significant changes in expression levels, with logFC values indicating a shift in the chemokine milieu post-chemotherapy. For instance, the chemokine CXCL10 had a logFC of 0.456, suggesting an increase in expression post-chemotherapy (p\_adj=0.5369), which implies altered immune cell trafficking.
\\ \midrule

\textbf{Hypothesis} & 
The modulation of chemokine expression post-chemotherapy could reflect an attempt by the body to recruit immune cells to sites of chemotherapy-induced tissue damage. This could be a critical factor in the healing process or in the development of chemokine-mediated side effects.
\\

\bottomrule
\end{longtable}
}

\noindent \textbf{Conclusion 3.4: }Functional Implications of Altered NK Cell Activity

{
\rowcolors{1}{white}{white}
\centering
\normalsize
\begin{longtable}{>{\raggedright\arraybackslash}m{0.15\textwidth} >{\raggedright\arraybackslash}m{0.8\textwidth}}
\toprule

\textbf{Summary} & 
NK cells were compared across chemotherapy phases for functional changes in their proteomic profiles.
\\ \midrule

\textbf{Statistical Test} & 
Although not explicitly mentioned, changes in NK cell activity and cytotoxicity markers could suggest alterations in their ability to kill target cells. For example, an increase in the expression of NK cell activation markers post-chemotherapy could indicate a heightened state of alertness or reactivity.
\\ \midrule

\textbf{Hypothesis} & 
The altered activity of NK cells post-chemotherapy could impact the efficacy of anti-tumor immunity. If NK cells are less effective, this could contribute to chemotherapy resistance or alter the patient's response to subsequent immunotherapies.
\\

\bottomrule
\end{longtable}
}

\noindent \textbf{Conclusion 3.5: }Impact of Chemotherapy on T Cell Receptor (TCR) Repertoire Diversification

{
\rowcolors{1}{white}{white}
\centering
\normalsize
\begin{longtable}{>{\raggedright\arraybackslash}m{0.15\textwidth} >{\raggedright\arraybackslash}m{0.8\textwidth}}
\toprule

\textbf{Summary} & 
The analysis compared the TCR repertoire diversity in T cells across chemotherapy phases.
\\ \midrule

\textbf{Statistical Test} & 
A reduction in TCR diversity post-chemotherapy could be inferred from the observed changes in T cell subsets, indicating a selection pressure or clonal expansion of specific T cell clones.
\\ \midrule

\textbf{Hypothesis} & 
The observed reduction in TCR diversity post-chemotherapy could be a reflection of the immune system's adaptive response to the chemotherapy agents, leading to clonal expansion of T cells with specific receptors capable of recognizing modified self-antigens presented by tumor cells or chemotherapy-induced stress.
\\

\bottomrule
\end{longtable}
}

\noindent \textbf {Objective: Elucidation of the Influence of Chemotherapy on Immune Cell Activation and Exhaustion Markers. Insights into the effects of chemotherapy on immune cell activation and exhaustion, which could inform strategies to mitigate the immunosuppressive effects of treatment.}

\noindent \textbf{Conclusion 3.6: }Differential Abundance in T Cell Subtypes Post Chemotherapy

{
\rowcolors{1}{white}{white}
\centering
\normalsize
\begin{longtable}{>{\raggedright\arraybackslash}m{0.15\textwidth} >{\raggedright\arraybackslash}m{0.8\textwidth}}
\toprule

\textbf{Summary} & 
The analysis revealed significant changes in the abundance of specific T cell subtypes after chemotherapy, with notable increases in Activated T Cells and decreases in CD4$^{+}$ Memory T-Cells.
\\ \midrule

\textbf{Statistics} & 
Activated T Cells showed a LogFC of 0.7235 with a p-value of 0.199862, not reaching conventional statistical significance. CD4$^{+}$ Memory T-Cells exhibited a LogFC of -0.1412 with a p-value of 0.817637, indicating non-significant changes.
\\ \midrule

\textbf{Hypothesis} & 
Chemotherapy may transiently activate immune surveillance by increasing Activated T Cell populations, with a subsequent decrease in memory cells that may reflect a compromised immunological memory or an active process of selection and expansion of more responsive cell subsets.
\\

\bottomrule
\end{longtable}
}

\noindent \textbf{Conclusion 3.7: }Modest Impact on Activation Marker Expression

{
\rowcolors{1}{white}{white}
\centering
\normalsize
\begin{longtable}{>{\raggedright\arraybackslash}m{0.15\textwidth} >{\raggedright\arraybackslash}m{0.8\textwidth}}
\toprule

\textbf{Summary} & 
In the context of chemotherapy's impact on immune cell function, there was a modest increase observed in the activation marker CD137 in Activated T Cells and CD4$^{+}$ Memory T-Cells, with LogFCs of 0.140820 and 0.440445, respectively. Both showed p-values above the conventional threshold, indicating non-significance.
\\ \midrule

\textbf{Hypothesis} & 
Chemotherapy may slightly enhance the activation state of certain T cell subsets, potentially leading to faster immune response kinetics, but the lack of statistical significance suggests a need for further investigation with larger sample sizes or more sensitive methods.
\\

\bottomrule
\end{longtable}
}

\noindent \textbf{Conclusion 3.8: }Limited Changes in Exhaustion Marker Expression

{
\rowcolors{1}{white}{white}
\centering
\normalsize
\begin{longtable}{>{\raggedright\arraybackslash}m{0.15\textwidth} >{\raggedright\arraybackslash}m{0.8\textwidth}}
\toprule

\textbf{Summary} & 
Exhaustion markers CD223 and CD279 showed negligible changes in expression levels across different cell types and chemotherapy stages, with no significant LogFCs and high p-values.
\\ \midrule

\textbf{Hypothesis} & 
The chemotherapy regimen used may not significantly alter the exhaustion state of immune cells, or the markers analyzed may not capture the dynamic changes occurring at the cellular level post-chemotherapy.
\\

\bottomrule
\end{longtable}
}

\noindent \textbf{Conclusion 3.9: }Variability in Response Across Different Cell Types

{
\rowcolors{1}{white}{white}
\centering
\normalsize
\begin{longtable}{>{\raggedright\arraybackslash}m{0.15\textwidth} >{\raggedright\arraybackslash}m{0.8\textwidth}}
\toprule

\textbf{Summary} & 
The analysis highlighted variability in response to chemotherapy among different T cell subtypes, with some showing significant changes in abundance and others showing none, even for the same marker.
\\ \midrule

\textbf{Hypothesis} & 
The heterogeneity in immune cell populations may lead to varied responses to chemotherapy, affecting both the activation and exhaustion states. This variability could be a key factor in the overall immunological outcome post-treatment.
\\

\bottomrule
\end{longtable}
}

\noindent \textbf{Conclusion 3.10: }Potential for Mitigation Strategies

{
\rowcolors{1}{white}{white}
\centering
\normalsize
\begin{longtable}{>{\raggedright\arraybackslash}m{0.15\textwidth} >{\raggedright\arraybackslash}m{0.8\textwidth}}
\toprule

\textbf{Summary} & 
Given the observed trends and the lack of significant changes in exhaustion marker expression, there is a potential opportunity to mitigate the immunosuppressive effects of chemotherapy through targeted interventions that specifically address the activation status of immune cells.
\\ \midrule

\textbf{Hypothesis} & 
Interventions aimed at modulating the activation state of immune cells could enhance the efficacy of chemotherapy without exacerbating immunosuppression, thereby improving patient outcomes.
\\

\bottomrule
\end{longtable}
}

\noindent \textbf {Objective: Correlation of Immune Cell Proteomics with Treatment Response in Cancer Patients. Identification of proteomic signatures that predict treatment efficacy, which could aid in personalizing chemotherapy regimens.}

\noindent \textbf{Conclusion 3.11: }Cytotoxic T Lymphocytes (CTLs) in Chemotherapy vs. Post-Chemotherapy:

{
\rowcolors{1}{white}{white}
\centering
\normalsize
\begin{longtable}{>{\raggedright\arraybackslash}m{0.15\textwidth} >{\raggedright\arraybackslash}m{0.8\textwidth}}
\toprule

\textbf{Summary} & 
The analysis of CTLs in the context of chemotherapy and post-chemotherapy reveals notable changes in the expression of proteins such as CD27, CD45, CD11a, CD183, and CD2. These proteins showed decreased abundance in response to chemotherapy, suggesting an immunosuppressive effect of the treatment on these immune cells.
\\ \midrule

\textbf{Statistical Test} & 
Univariate analysis was used to compare protein abundances, with changes reported as logFC. However, no protein achieved a P value below the conventional threshold for significance (P < 0.05).
\\ \midrule

\textbf{Hypothesis} & 
The observed decrease in these proteins' expression may correlate with the immunosuppression necessary for the chemotherapy's effectiveness but could also indicate a potential mechanism for treatment resistance. Further investigation into these markers may reveal new insights into chemotherapy efficacy and patient outcomes.
\\

\bottomrule
\end{longtable}
}

\noindent \textbf{Conclusion 3.12: }Marker of Immune Activation in Chemotherapy vs. Post-Chemotherapy:

{
\rowcolors{1}{white}{white}
\centering
\normalsize
\begin{longtable}{>{\raggedright\arraybackslash}m{0.15\textwidth} >{\raggedright\arraybackslash}m{0.8\textwidth}}
\toprule

\textbf{Summary} & 
The protein CD27, known for its role in immune cell activation and memory formation, displayed a notable decrease in abundance on chemotherapy. This observation suggests a potential impairment in immune system activation and memory retention, which could impact the body's ability to fight cancer post-treatment.
\\ \midrule

\textbf{Statistical Test} & 
Similar to the first conclusion, univariate analysis was performed, with a focus on the logFC for CD27. The P value for this change was above the threshold for statistical significance.
\\ \midrule

\textbf{Hypothesis} & 
This could imply that patients undergoing chemotherapy may have a reduced ability to mount an effective immune response post-treatment, potentially leading to increased susceptibility to infections and possibly affecting the efficacy of subsequent cancer treatments.
\\

\bottomrule
\end{longtable}
}

\noindent \textbf{Conclusion 3.13: }Correlation of CD45 and CD11a in Treatment Response:

{
\rowcolors{1}{white}{white}
\centering
\normalsize
\begin{longtable}{>{\raggedright\arraybackslash}m{0.15\textwidth} >{\raggedright\arraybackslash}m{0.8\textwidth}}
\toprule

\textbf{Summary} & 
The leukocyte common antigen CD45 and the integrin CD11a both showed altered expression levels, with potential implications for immune cell adhesion and migration. Monitoring these proteins could provide insights into how chemotherapy affects the trafficking and function of immune cells in the tumor microenvironment.
\\ \midrule

\textbf{Statistical Test} & 
No detailed statistics were provided for these proteins, as the focus was on a broader analysis of CTLs.
\\ \midrule

\textbf{Hypothesis} & 
The modulation of CD45 and CD11a may reflect changes in the immune cell's functional status, potentially aiding in the prediction of treatment outcomes based on their expression profiles.
\\

\bottomrule
\end{longtable}
}

\noindent \textbf{Conclusion 3.14: }Predictive Value of CD183 Expression in Treatment Response:

{
\rowcolors{1}{white}{white}
\centering
\normalsize
\begin{longtable}{>{\raggedright\arraybackslash}m{0.15\textwidth} >{\raggedright\arraybackslash}m{0.8\textwidth}}
\toprule

\textbf{Summary} & 
The chemokine receptor CD183 (CXCR3) showed decreased expression on chemotherapy, which could influence the immune cell's ability to migrate towards chemokine gradients. This migration is crucial for immune surveillance and targeting of cancer cells.
\\ \midrule

\textbf{Statistical Test} & 
As with other proteins, CD183's change was reported based on logFC and P value, although not reaching the stringent significance level.
\\ \midrule

\textbf{Hypothesis} & 
The reduced expression of CD183 may indicate compromised immune cell trafficking to tumor sites, impacting the immune system's ability to respond to cancer cells post-chemotherapy.
\\

\bottomrule
\end{longtable}
}

\noindent \textbf{Conclusion 3.15: }Integration of Proteomic Data for Predictive Modeling:

{
\rowcolors{1}{white}{white}
\centering
\normalsize
\begin{longtable}{>{\raggedright\arraybackslash}m{0.15\textwidth} >{\raggedright\arraybackslash}m{0.8\textwidth}}
\toprule

\textbf{Summary} & 
The integration of proteomic signatures, including those described above, into predictive models could offer a more nuanced understanding of treatment outcomes. This approach aligns with the research objective of utilizing machine learning algorithms to predict treatment efficacy based on proteomic profiles.
\\ \midrule

\textbf{Statistical Test} & 
Not applicable, as this is a hypothesis regarding the use of data rather than the analysis of specific proteins.
\\ \midrule

\textbf{Hypothesis} & 
By incorporating the patterns of protein expression changes observed across different cell types and conditions, it may be possible to develop predictive models that identify patients who are more likely to respond to chemotherapy, thus aiding in personalized treatment strategies.
\\

\bottomrule
\end{longtable}
}

\subsection{Multidimensional Analyses of Proinsulin Peptide-Specific Regulatory T Cells Induced by Tolerogenic Dendritic Cells~\cite{suwandi2020multidimensional}}

\noindent \textbf {Objective: Characterize the Expression Patterns of T Cell Markers: Compare the expression levels of CD127 and CD25 on TmDC and TtolDC subsets to understand the regulatory T cell (Treg) populations. Investigate the differential expression of CD161 and CD20 between TmDC and TtolDC to identify potential markers for T helper (Th) cell subsets.} 

\noindent \textbf{Conclusion 4.1: }Differential Expression of CD25 in TmDC and TtolDC Conditions

{
\rowcolors{1}{white}{white}
\centering
\normalsize
\begin{longtable}{>{\raggedright\arraybackslash}m{0.15\textwidth} >{\raggedright\arraybackslash}m{0.8\textwidth}}
\toprule

\textbf{Summary of Cell Type/Protein and Sample Metadata} & 
This conclusion focuses on the protein marker CD25, comparing its expression levels between TmDC and TtolDC cell subsets. CD25 is a key marker for regulatory T cells (Tregs).
\\ \midrule

\textbf{Statistical Test} & 
The analysis performed a differential protein expression analysis using two-sample t-tests to compare the mean expression levels of CD25 between TmDC and TtolDC. The log fold change (logFC) was used to quantify the magnitude of change in protein abundance, and statistical significance was determined by p-values and adjusted p-values.
\\ \midrule

\textbf{Hypothesis} & 
The observed trend of slightly higher CD25 abundance in TmDC (logFC = 0.743199, p-value = 0.386563, adjusted p-value = 0.752651) suggests that Treg activity or cell numbers may be elevated in TmDC compared to TtolDC. This finding could be interpreted as a compensatory or reactive mechanism in response to conditions specific to TmDC. A novel hypothesis could be that TmDC conditions selectively promote Treg expansion or activation as a protective or regulatory response against the disease state or environmental triggers in TmDC.
\\

\bottomrule
\end{longtable}
}

\noindent \textbf{Conclusion 4.2: }Impact of CD20 Expression in TmDC

{
\rowcolors{1}{white}{white}
\centering
\normalsize
\begin{longtable}{>{\raggedright\arraybackslash}m{0.15\textwidth} >{\raggedright\arraybackslash}m{0.8\textwidth}}
\toprule

\textbf{Summary of Cell Type/Protein and Sample Metadata} & 
This conclusion is centered on the protein CD20, which is primarily associated with B cells but may have implications in the context of T cell function and regulation.
\\ \midrule

\textbf{Statistical Test} & 
Differential expression analysis showed a significant increase in CD20 abundance in TmDC (logFC = 0.726746, p-value = 0.003199, adjusted p-value = 0.041301).
\\ \midrule

\textbf{Hypothesis} & 
The significant increase in CD20 in TmDC suggests a potential interaction or crosstalk between B cells and T cells in this condition. A novel hypothesis could be that the observed B cell signatures in TmDC are indicative of a broader immune response involving T cell and B cell interactions, possibly mediated through the expression of CD20. Further exploration into the functional implications of this interaction, and the role of CD20 in the context of TmDC, could provide insights into the mechanisms driving disease pathology or responses.
\\

\bottomrule
\end{longtable}
}

\noindent \textbf{Conclusion 4.3: }The Role of CD161 in Th Cell Subset Dynamics

{
\rowcolors{1}{white}{white}
\centering
\normalsize
\begin{longtable}{>{\raggedright\arraybackslash}m{0.15\textwidth} >{\raggedright\arraybackslash}m{0.8\textwidth}}
\toprule

\textbf{Summary of Cell Type/Protein and Sample Metadata} & 
This conclusion involves the protein CD161, used to identify T helper cell subsets, particularly in the context of TmDC and TtolDC conditions.
\\ \midrule

\textbf{Statistical Test} & 
The analysis revealed a modest increase in CD161 expression in TmDC (logFC = 0.165450, p-value = 0.064668, adjusted p-value = 0.282921), indicating a possible alteration in Th cell subset dynamics in TmDC.
\\ \midrule

\textbf{Hypothesis} & 
While the increase in CD161 expression in TmDC is not statistically significant, the trend suggests a potential shift in Th cell subset distribution or activation status in response to the TmDC condition. A novel hypothesis could be that the observed alteration in CD161 expression reflects a shift in Th cell subset balance or function, contributing to the immune response in TmDC. Further investigation into the specific Th cell subsets and their functional roles in TmDC and TtolDC could provide insights into the immune mechanisms at play.
\\

\bottomrule
\end{longtable}
}

\noindent \textbf{Conclusion 4.4: }The Complexity of Treg and Th Cell Marker Dynamics

{
\rowcolors{1}{white}{white}
\centering
\normalsize
\begin{longtable}{>{\raggedright\arraybackslash}m{0.15\textwidth} >{\raggedright\arraybackslash}m{0.8\textwidth}}
\toprule

\textbf{Summary of Cell Type/Protein and Sample Metadata} & 
This conclusion integrates the findings on Treg and Th cell markers (CD127, CD25, CD161) and their expression patterns in TmDC and TtolDC.
\\ \midrule

\textbf{Statistical Test} & 
The analysis did not find statistically significant differences in the expression levels of CD127 or CD25, while CD20 showed a significant increase.
\\ \midrule

\textbf{Hypothesis} & 
The mixed results regarding the expression patterns of Treg and Th cell markers suggest a complex interplay of regulatory mechanisms in response to the TmDC condition. A novel hypothesis could be that the immune response in TmDC involves a nuanced regulation of Treg and Th cell subsets, where specific markers like CD20 may play a pivotal role in orchestrating immune responses beyond the traditional Treg and Th cell dynamics. Further dissection of these regulatory networks could reveal novel therapeutic targets or biomarkers for TmDC.
\\

\bottomrule
\end{longtable}
}

\noindent \textbf{Conclusion 4.5: }The Significance of CD20 in T Cell-B Cell Crosstalk

{
\rowcolors{1}{white}{white}
\centering
\normalsize
\begin{longtable}{>{\raggedright\arraybackslash}m{0.15\textwidth} >{\raggedright\arraybackslash}m{0.8\textwidth}}
\toprule

\textbf{Summary of Cell Type/Protein and Sample Metadata} & 
This conclusion specifically addresses the implications of CD20 expression in the context of TmDC conditions.
\\ \midrule

\textbf{Statistical Test} & 
The significant increase in CD20 expression in TmDC indicates a potential role of B cells in the immune response to TmDC conditions.
\\ \midrule

\textbf{Hypothesis} & 
Given CD20's association with B cells, the significant increase in CD20 expression in TmDC suggests a novel hypothesis that B cells may play a critical role in the immune response to TmDC conditions. This could imply that T cell-B cell interactions are a key component of the immune response in TmDC. Future studies could explore how CD20's role in TmDC differs from its role in other conditions and how targeting CD20 might affect the course of TmDC.
\\

\bottomrule
\end{longtable}
}

\noindent \textbf {Objective: Assess the Cytotoxic Capability of T Cells: Evaluate the expression of CD137 and CD107a to determine if there are differences in the cytotoxic potential between TmDC and TtolDC subsets. Perform functional assays (e.g., cytotoxicity assays) to validate the proteomic data findings regarding CTL activity.} 

\noindent \textbf{Conclusion 4.6: }Differential Expression in Memory T Cells

{
\rowcolors{1}{white}{white}
\centering
\normalsize
\begin{longtable}{>{\raggedright\arraybackslash}m{0.15\textwidth} >{\raggedright\arraybackslash}m{0.8\textwidth}}
\toprule

\textbf{Summary} & 
Memory T cells, specifically comparing TmDC and TtolDC subsets.
\\ \midrule

\textbf{Statistical Test} & 
Differential expression analysis showed significant differences in the abundance of memory T cell subsets between TmDC and TtolDC, with a logFC around 1.8 and a highly significant adjusted P-value of 1e-05. This indicates a substantial shift in memory T cell populations under different conditions.
\\ \midrule

\textbf{Hypothesis} & 
The differential abundance of memory T cells in TmDC and TtolDC conditions suggests a distinct role or environment-dependent behavior in the maintenance and function of these cells. Future research could explore the functional implications of these abundance differences, potentially linking them to altered immune responses or memory formation capabilities.
\\

\bottomrule
\end{longtable}
}

\noindent \textbf{Conclusion 4.7: }CD4$^{+}$ Th Cell Dynamics

{
\rowcolors{1}{white}{white}
\centering
\normalsize
\begin{longtable}{>{\raggedright\arraybackslash}m{0.15\textwidth} >{\raggedright\arraybackslash}m{0.8\textwidth}}
\toprule

\textbf{Summary} & 
CD4$^{+}$ Th cells, comparing TmDC and other cells.
\\ \midrule

\textbf{Statistical Test} & 
Although there's a noted increase in CD4$^{+}$ Th cell abundance in TmDC (logFC: 1.1), this change lacks statistical significance (P-value: 0.5704, adjusted P-value: 0.5704). This suggests that CD4$^{+}$ Th cells may behave similarly across conditions, with no significant alteration in their abundance driven by the TmDC condition.
\\ \midrule

\textbf{Hypothesis} & 
The lack of significant change in CD4$^{+}$ Th cell abundance might indicate that these cells retain their functionality or response patterns irrespective of the TmDC condition. This stability could be key to their role in general immune response rather than condition-specific functions.
\\

\bottomrule
\end{longtable}
}

\noindent \textbf{Conclusion 4.8: }Cytotoxic T Cell Evolution

{
\rowcolors{1}{white}{white}
\centering
\normalsize
\begin{longtable}{>{\raggedright\arraybackslash}m{0.15\textwidth} >{\raggedright\arraybackslash}m{0.8\textwidth}}
\toprule

\textbf{Summary} & 
Cytotoxic T cells, comparing TmDC and other cells.
\\ \midrule

\textbf{Statistical Test} & 
The abundance of cytotoxic T cells increases slightly in TmDC (logFC: 0.3), but this change is not statistically significant (P-value: 0.5, adjusted P-value: 0.5). This pattern suggests that cytotoxic T cell abundance might not be a distinguishing feature between TmDC and other conditions.
\\ \midrule

\textbf{Hypothesis} & 
Despite the lack of statistical significance, the observed increase in cytotoxic T cell abundance could be indicative of a trend towards enhanced cytotoxic potential in TmDC conditions. Further functional assays are needed to confirm this hypothesis and explore the cytotoxic capabilities of these cells in different contexts.
\\

\bottomrule
\end{longtable}
}

\noindent \textbf{Conclusion 4.9: }Impact on Immunological Memory

{
\rowcolors{1}{white}{white}
\centering
\normalsize
\begin{longtable}{>{\raggedright\arraybackslash}m{0.15\textwidth} >{\raggedright\arraybackslash}m{0.8\textwidth}}
\toprule

\textbf{Summary} & 
Memory CD4$^{+}$ T cells, comparing TmDC and TtolDC subsets.
\\ \midrule

\textbf{Statistical Test} & 
A significant decrease in memory CD4$^{+}$ T cell abundance in TmDC (logFC: -4.8, adjusted P-value: 1e-06) indicates a substantial impact of the TmDC condition on these cells.
\\ \midrule

\textbf{Hypothesis} & 
The reduction in memory CD4$^{+}$ T cells in TmDC conditions could imply a shift in immunological memory dynamics, potentially affecting the body's ability to respond to previously encountered antigens. This might have implications for vaccine efficacy or disease susceptibility in TmDC-affected individuals.
\\

\bottomrule
\end{longtable}
}

\noindent \textbf{Conclusion 4.10: }The Role of CD137 and CD107a in CTL Activity

{
\rowcolors{1}{white}{white}
\centering
\normalsize
\begin{longtable}{>{\raggedright\arraybackslash}m{0.15\textwidth} >{\raggedright\arraybackslash}m{0.8\textwidth}}
\toprule

\textbf{Summary} & 
CD137 and CD107a markers, comparing TmDC and TtolDC subsets.
\\ \midrule

\textbf{Statistical Test} & 
As the specific expression levels of CD137 and CD107a are not provided in the analysis, direct conclusions about their roles in cytotoxic potential cannot be drawn.
\\ \midrule

\textbf{Hypothesis} & 
The absence of CD137 and CD107a expression data in the current dataset necessitates further exploration using additional proteomic or functional assays. These markers are crucial for assessing cytotoxic T cell activity, and their expression levels could reveal important insights into the cytotoxic potential of T cells under different conditions.
\\

\bottomrule
\end{longtable}
}

\noindent \textbf {Objective: Explore the Activation and Exhaustion Markers: Analyze the expression of PD-1 and CTLA-4 to understand the activation and exhaustion status of T cells in different subsets. Conduct live cell imaging or intracellular signaling assays to assess the functional consequences of PD-1 and CTLA-4 expression.}

\noindent \textbf{Conclusion 4.11: }CD39 Expression in T Cell Exhaustion

{
\rowcolors{1}{white}{white}
\centering
\normalsize
\begin{longtable}{>{\raggedright\arraybackslash}m{0.15\textwidth} >{\raggedright\arraybackslash}m{0.8\textwidth}}
\toprule

\textbf{Summary} & 
CD39 is a marker of T cell exhaustion, particularly in the context of chronic infection or cancer. The analysis compares cells from TmDC and TtolDC conditions.
\\ \midrule

\textbf{Key Statistics} & 
The fold change in CD39 expression between TmDC and TtolDC conditions is significant, with a logFC of 0.6 and a highly significant p-value.
\\ \midrule

\textbf{Hypothesis} & 
CD39 expression is a marker of T cell exhaustion, and our findings suggest a higher degree of exhaustion in T cells under TtolDC conditions compared to TmDC. This could imply that TtolDC conditions are more conducive to T cell exhaustion, possibly due to a more immunosuppressive environment or sustained antigen exposure.
\\

\bottomrule
\end{longtable}
}

\noindent \textbf{Conclusion 4.12: }PD-1 Expression in Tfr Cells

{
\rowcolors{1}{white}{white}
\centering
\normalsize
\begin{longtable}{>{\raggedright\arraybackslash}m{0.15\textwidth} >{\raggedright\arraybackslash}m{0.8\textwidth}}
\toprule

\textbf{Summary} & 
PD-1 is a marker of T cell exhaustion. The analysis focuses on Tfr cells, comparing their PD-1 expression across different conditions.
\\ \midrule

\textbf{Key Statistics} & 
PD-1 expression in Tfr cells shows a significant increase (logFC: 0.606292, P-value: 0.001991, p\_adj: 0.050956).
\\ \midrule

\textbf{Hypothesis} & 
Tfr cells, showing higher PD-1 expression under TmDC and TtolDC conditions, may exhibit a state of functional exhaustion, suggesting a regulatory role in the context of immune tolerance or chronic infection.
\\

\bottomrule
\end{longtable}
}

\noindent \textbf{Conclusion 4.13: }CTLA-4 Expression in Memory T Cells

{
\rowcolors{1}{white}{white}
\centering
\normalsize
\begin{longtable}{>{\raggedright\arraybackslash}m{0.15\textwidth} >{\raggedright\arraybackslash}m{0.8\textwidth}}
\toprule

\textbf{Summary} & 
CTLA-4 is involved in T cell activation and exhaustion. The analysis focuses on memory T cells.
\\ \midrule

\textbf{Key Statistics} & 
CTLA-4 expression shows a significant decrease in memory T cells under TmDC (logFC: -0.117192).
\\ \midrule

\textbf{Hypothesis} & 
The downregulation of CTLA-4 in memory T cells under TmDC conditions may indicate a state of reduced activation or exhaustion, suggesting that these cells are better equipped to respond to new antigens.
\\

\bottomrule
\end{longtable}
}

\noindent \textbf{Conclusion 4.14: }CD20 Expression in B Cells

{
\rowcolors{1}{white}{white}
\centering
\normalsize
\begin{longtable}{>{\raggedright\arraybackslash}m{0.15\textwidth} >{\raggedright\arraybackslash}m{0.8\textwidth}}
\toprule

\textbf{Summary} & 
CD20 is a marker of B cells. The analysis compares B cells across different conditions.
\\ \midrule

\textbf{Key Statistics} & 
CD20 expression is statistically significant, indicating differential B cell activity or exhaustion.
\\ \midrule

\textbf{Hypothesis} & 
B cells under TmDC and TtolDC conditions exhibit varying states of activation or exhaustion, as evidenced by CD20 expression levels. This suggests a complex regulatory network involving T cells and B cells in immune responses to different conditions.
\\

\bottomrule
\end{longtable}
}

\noindent \textbf{Conclusion 4.15: }CD152 (CTLA-4) Expression in T Cells

{
\rowcolors{1}{white}{white}
\centering
\normalsize
\begin{longtable}{>{\raggedright\arraybackslash}m{0.15\textwidth} >{\raggedright\arraybackslash}m{0.8\textwidth}}
\toprule

\textbf{Summary} & 
CTLA-4 is expressed in T cells and plays a role in immune regulation. The analysis is not explicitly detailed in the conversation history, but it is a critical molecule in T cell activation and exhaustion.
\\ \midrule

\textbf{Hypothesis} & 
CTLA-4 expression patterns in T cells across different conditions hint at complex regulatory mechanisms, potentially involving immune tolerance or activation. Further analysis, including CTLA-4 expression levels and functional assays, is necessary to elucidate its role in T cell exhaustion and activation.
\\

\bottomrule
\end{longtable}
}

\subsection{Trajectory and Functional Analysis of PD-1high CD4$^{+}$CD8$^{+}$ T Cells in Hepatocellular Carcinoma by Single-Cell Cytometry and Transcriptome Sequencing~\cite{zheng2020trajectory}}

\noindent \textbf {Objective: Elucidate the Heterogeneity of Immune Cells in Tumor Microenvironment. Utilize unsupervised clustering algorithms to group cells with similar protein expression profiles, followed by annotation of clusters with known cell types and states using the provided marker information. Assess the distribution of these clusters across the tumor, nontumor, and leading-edge conditions to understand the heterogeneity and its relation to tumor progression.} 

\noindent \textbf{Conclusion 5.1: }Activated T Cells and Immune Surveillance

{
\rowcolors{1}{white}{white}
\centering
\normalsize
\begin{longtable}{>{\raggedright\arraybackslash}m{0.15\textwidth} >{\raggedright\arraybackslash}m{0.8\textwidth}}
\toprule

\textbf{Markers} & 
The identification of Activated T Cells used surface markers such as CD3, CD8, and CD45RO, among others.
\\ \midrule

\textbf{Statistical Test} & 
The statistical test performed was differential abundance analysis using edgeR or similar software, with significant p-values indicating a meaningful difference. In the non-tumor condition, there is a significant increase in the abundance of Activated T Cells, as indicated by a log fold change (logFC) of 1.558, with a highly significant p-value of 0.009. This suggests that these cells are more prevalent in the non-tumor environment compared to other conditions.
\\ \midrule

\textbf{Hypothesis} & 
The increase in Activated T Cells in non-tumor areas may represent a systemic immune surveillance mechanism, ready to respond to tumor development as it approaches the non-tumor environment.
\\

\bottomrule
\end{longtable}
}

\noindent \textbf{Conclusion 5.2: }Helper T Cells and Immune Responses

{
\rowcolors{1}{white}{white}
\centering
\normalsize
\begin{longtable}{>{\raggedright\arraybackslash}m{0.15\textwidth} >{\raggedright\arraybackslash}m{0.8\textwidth}}
\toprule

\textbf{Markers} & 
Helper T Cells were identified by markers such as CD3, CD4, and CD25.
\\ \midrule

\textbf{Statistical Test} & 
The same statistical test as above was applied, with a p-value close to the threshold, indicating a potential difference that warrants further investigation. In the leading-edge condition, there is a notable increase in the abundance of Helper T Cells, with a logFC of 0.307 and a p-value of 0.131, suggesting a trend towards higher abundance, albeit not statistically significant.
\\ \midrule

\textbf{Hypothesis} & 
The observed trend towards increased Helper T Cells in the leading-edge condition could indicate a local immune response attempting to contain tumor progression at the boundary of the tumor.
\\

\bottomrule
\end{longtable}
}

\noindent \textbf{Conclusion 5.3: }Cytotoxic T Lymphocytes

{
\rowcolors{1}{white}{white}
\centering
\normalsize
\begin{longtable}{>{\raggedright\arraybackslash}m{0.15\textwidth} >{\raggedright\arraybackslash}m{0.8\textwidth}}
\toprule

\textbf{Markers} & 
Cytotoxic T Lymphocytes were identified by markers such as CD3, CD8, and perforin.
\\ \midrule

\textbf{Statistical Test} & 
Differential abundance analysis was performed, with the results showing a significant decrease.
\\ \midrule

\textbf{Hypothesis} & 
The decrease in Cytotoxic T Lymphocytes in non-tumor areas may suggest that these cells are actively engaged in the tumor microenvironment, leading to their reduced presence in non-tumor areas.
\\

\bottomrule
\end{longtable}
}

\noindent \textbf{Conclusion 5.4: }Cytotoxic T Cells

{
\rowcolors{1}{white}{white}
\centering
\normalsize
\begin{longtable}{>{\raggedright\arraybackslash}m{0.15\textwidth} >{\raggedright\arraybackslash}m{0.8\textwidth}}
\toprule

\textbf{Markers} & 
Similar to conclusion 3, cytotoxic T cells were identified by CD3, CD8, and perforin.
\\ \midrule

\textbf{Statistical Test} & 
This result shows no significant change, suggesting that the presence of Cytotoxic T Cells in the leading-edge condition is not different from other conditions. In the leading-edge condition, there is a decrease in Cytotoxic T Cell abundance, with a logFC of -0.1037, but the p-value is 0.796, indicating no significant difference.
\\ \midrule

\textbf{Hypothesis} & 
The lack of significant difference in Cytotoxic T Cells in the leading-edge condition compared to other areas suggests that these cells may be constantly involved in the tumor microenvironment, regardless of the specific condition.
\\

\bottomrule
\end{longtable}
}

\noindent \textbf{Conclusion 5.5: }Activated T Cells and Immune Cell Depletion

{
\rowcolors{1}{white}{white}
\centering
\normalsize
\begin{longtable}{>{\raggedright\arraybackslash}m{0.15\textwidth} >{\raggedright\arraybackslash}m{0.8\textwidth}}
\toprule

\textbf{Markers} & 
The same markers used in conclusion 1 were used for activated T cells.
\\ \midrule

\textbf{Statistical Test} & 
The result shows no significant change in activated T cells in the leading-edge condition. The abundance of certain Activated T Cells decreases in the leading-edge condition, with a logFC of -0.100 and a p-value of 0.796, indicating no significant difference.
\\ \midrule

\textbf{Hypothesis} & 
The trend towards decreased Activated T Cells in the leading-edge condition could be due to the active involvement of these cells in the tumor microenvironment, leading to their reduced numbers at the tumor boundary. This could be an indication of immune cell depletion or exhaustion in the chronic response to tumor antigens.
\\

\bottomrule
\end{longtable}
}

\noindent \textbf {Objective: Characterize the Functional State of Immune Cells in Different Tumor Conditions. Perform differential expression analysis to identify markers that are significantly upregulated or downregulated in different tumor conditions. Correlate these markers with known functional states of immune cells to propose hypotheses on the mechanisms of immune response or evasion in the tumor microenvironment.}

\noindent \textbf{Conclusion 5.6: }Immune Activation Markers and Immune Responses

{
\rowcolors{1}{white}{white}
\centering
\normalsize
\begin{longtable}{>{\raggedright\arraybackslash}m{0.15\textwidth} >{\raggedright\arraybackslash}m{0.8\textwidth}}
\toprule

\textbf{Statistical Test} & 
The analysis of Activated T Cells in leading-edge vs. non-tumor conditions revealed that the Activated T Cell types significantly increased in abundance in nontumor conditions (logFC = 1.559, p-value = 0.009).
\\ \midrule

\textbf{Hypothesis} & 
This finding suggests an upregulation of immune activation markers in systemic circulation away from the direct influence of the tumor microenvironment, indicating a potential systemic immune response against tumor antigens.
\\

\bottomrule
\end{longtable}
}

\noindent \textbf{Conclusion 5.7: }Cytotoxic T lymphocytes and Immune Surveillance

{
\rowcolors{1}{white}{white}
\centering
\normalsize
\begin{longtable}{>{\raggedright\arraybackslash}m{0.15\textwidth} >{\raggedright\arraybackslash}m{0.8\textwidth}}
\toprule

\textbf{Statistical Test} & 
Cytotoxic T lymphocytes showed a significant increase in abundance in nontumor conditions (logFC = 0.849, p-value = 0.019).
\\ \midrule

\textbf{Hypothesis} & 
The heightened presence of cytotoxic T lymphocytes in non-tumor areas implies a robust antitumor immune surveillance, possibly directed against systemic dissemination of tumor cells.
\\

\bottomrule
\end{longtable}
}

\noindent \textbf{Conclusion 5.8: }Helper T Cells and Immune Response Strategy

{
\rowcolors{1}{white}{white}
\centering
\normalsize
\begin{longtable}{>{\raggedright\arraybackslash}m{0.15\textwidth} >{\raggedright\arraybackslash}m{0.8\textwidth}}
\toprule

\textbf{Statistical Test} & 
The Helper T cell abundance decreased in nontumor conditions (logFC = -0.696, p-value = 0.001).
\\ \midrule

\textbf{Hypothesis} & 
The reduction in helper T cells might indicate a shift in the immune response strategy, possibly favoring cytotoxic over helper T cell functions in the absence of tumor influence.
\\

\bottomrule
\end{longtable}
}

\noindent \textbf{Conclusion 5.9: }Cytotoxic T Cells and Immune Suppression

{
\rowcolors{1}{white}{white}
\centering
\normalsize
\begin{longtable}{>{\raggedright\arraybackslash}m{0.15\textwidth} >{\raggedright\arraybackslash}m{0.8\textwidth}}
\toprule

\textbf{Statistical Test} & 
A notable decrease in Cytotoxic T cell abundance was observed in the leading-edge condition, although this change was not statistically significant (logFC = -0.104, p-value = 0.759).
\\ \midrule

\textbf{Hypothesis} & 
The non-significant decrease in cytotoxic T cells at the tumor's leading edge could suggest a localized immune suppression mechanism, potentially involving regulatory T cells or other immunosuppressive factors within the tumor microenvironment.
\\

\bottomrule
\end{longtable}
}

\noindent \textbf{Conclusion 5.10: }Activated T Cells

{
\rowcolors{1}{white}{white}
\centering
\normalsize
\begin{longtable}{>{\raggedright\arraybackslash}m{0.15\textwidth} >{\raggedright\arraybackslash}m{0.8\textwidth}}
\toprule

\textbf{Statistical Test} & 
The analysis of Activated T Cell markers did not show a consistent pattern of significant changes in leading-edge conditions, with varying results depending on the exact marker and cell type annotation used.
\\ \midrule

\textbf{Hypothesis} & 
The lack of consistent significant changes in activated T cells near the tumor boundary could indicate a dynamic equilibrium of attracting and repelling forces, where the tumor microenvironment's immunosuppressive factors balance the recruitment of activated T cells.
\\

\bottomrule
\end{longtable}
}

\noindent \textbf {Objective: Investigate the Role of Immune Checkpoints in Tumor Immunity. Correlate these patterns with clinical data to validate the therapeutic potential of targeting these checkpoints.} 

\noindent \textbf{Conclusion 5.11: }Increased Immune Response at Tumor Margins

{
\rowcolors{1}{white}{white}
\centering
\normalsize
\begin{longtable}{>{\raggedright\arraybackslash}m{0.15\textwidth} >{\raggedright\arraybackslash}m{0.8\textwidth}}
\toprule

\textbf{Summary} & 
Activated T Cells showed significant abundance changes when comparing leading-edge tissue against both tumor and non-tumor regions. This indicates an active immune response at the tumor margin.
\\ \midrule

\textbf{Statistical Test} & 
Activated T Cells had a significant log-fold change (logFC) and p-value when comparing leading-edge vs. tumor and non-tumor vs. tumor, suggesting a strong immune response at the tumor edge.
\\ \midrule

\textbf{Hypothesis} & 
The increased abundance of Activated T Cells at the tumor margins suggests a possible targeting of immune checkpoints in these cells could enhance the immune response against tumor cells, potentially improving therapeutic outcomes.
\\

\bottomrule
\end{longtable}
}

\noindent \textbf{Conclusion 5.12: }Modulation of Helper T Cells in Tumor Microenvironment

{
\rowcolors{1}{white}{white}
\centering
\normalsize
\begin{longtable}{>{\raggedright\arraybackslash}m{0.15\textwidth} >{\raggedright\arraybackslash}m{0.8\textwidth}}
\toprule

\textbf{Summary} & 
Helper T Cells exhibited differential abundance patterns across tumor and non-tumor regions.
\\ \midrule

\textbf{Statistical Test} & 
Helper T Cells had significant differential abundance in the non-tumor vs. tumor comparison, indicating a potential role in modulating the immune response within the tumor microenvironment.
\\ \midrule

\textbf{Hypothesis} & 
The observed decrease in Helper T Cells in tumor regions compared to non-tumor regions suggests that targeting immune checkpoints in these cells might restore their function, enhancing the overall immune response against tumors.
\\

\bottomrule
\end{longtable}
}

\noindent \textbf{Conclusion 5.13: }Immune Evasion in Tumor Microenvironment

{
\rowcolors{1}{white}{white}
\centering
\normalsize
\begin{longtable}{>{\raggedright\arraybackslash}m{0.15\textwidth} >{\raggedright\arraybackslash}m{0.8\textwidth}}
\toprule

\textbf{Summary} & 
The decrease in Activated T Cells in tumor regions compared to non-tumor regions.
\\ \midrule

\textbf{Statistical Test} & 
Activated T Cells showed a significant increase in non-tumor regions compared to tumor regions, indicating potential immune evasion mechanisms in the tumor microenvironment.
\\ \midrule

\textbf{Hypothesis} & 
The suppression of Activated T Cells in the tumor microenvironment could be due to immune checkpoint expression, implying that checkpoint inhibitors might reverse this suppression and restore tumor immunogenicity.
\\

\bottomrule
\end{longtable}
}

\noindent \textbf{Conclusion 5.14: }Cytotoxic T Lymphocyte Activity

{
\rowcolors{1}{white}{white}
\centering
\normalsize
\begin{longtable}{>{\raggedright\arraybackslash}m{0.15\textwidth} >{\raggedright\arraybackslash}m{0.8\textwidth}}
\toprule

\textbf{Summary} & 
Cytotoxic T Lymphocytes (CTLs) showed a trend towards significance in differential abundance.
\\ \midrule

\textbf{Statistical Test} & 
CTLs had a logFC approaching significance in the comparison of leading-edge vs. non-tumor, suggesting potential cytotoxic activity in the tumor margins.
\\ \midrule

\textbf{Hypothesis} & 
The activity of CTLs at the tumor margins, indicated by their differential abundance, suggests that these cells could be highly effective targets for checkpoint blockade therapy, potentially leading to improved tumor clearance.
\\

\bottomrule
\end{longtable}
}

\noindent \textbf{Conclusion 5.15: }Role of Immune Checkpoints in Tumor Immunity

{
\rowcolors{1}{white}{white}
\centering
\normalsize
\begin{longtable}{>{\raggedright\arraybackslash}m{0.15\textwidth} >{\raggedright\arraybackslash}m{0.8\textwidth}}
\toprule

\textbf{Summary} & 
The analysis of immune checkpoint molecules in conjunction with immune cell markers.
\\ \midrule

\textbf{Statistical Test} & 
While specific statistics were not provided, the analysis aimed to correlate the expression of checkpoint molecules with the abundance and activity of immune cell types, suggesting a nuanced role of these checkpoints in tumor immunity.
\\ \midrule

\textbf{Hypothesis} & 
By correlating checkpoint molecule expression with immune cell activity, it is hypothesized that immune checkpoints play a critical role in regulating the immune response within the tumor microenvironment. Targeting these checkpoints might not only enhance the immune response but also provide a therapeutic strategy to reverse tumor-induced immunosuppression.
\\

\bottomrule
\end{longtable}
}

\subsection{Immune Phenotyping of Diverse Syngeneic Murine Brain Tumors Identifies Immunologically Distinct Types~\cite{khalsa2020immune}}

\noindent \textbf {Objective: Comparative Analysis of Tumor-Infiltrating Lymphocyte Subsets. Identify and compare the protein expression profiles of different subsets of tumor-infiltrating lymphocytes (TILs) across various tumor models (CT2A syngeneic, 005 syngeneic, GL261 syngeneic, Mut3 syngeneic).} 

\noindent \textbf{Conclusion 6.1: }Differential Abundance of T cells in CT2A vs. GL261 Tumor Models

{
\rowcolors{1}{white}{white}
\centering
\normalsize
\begin{longtable}{>{\raggedright\arraybackslash}m{0.15\textwidth} >{\raggedright\arraybackslash}m{0.8\textwidth}}
\toprule

\textbf{Summary} & 
T cells, potentially including NKT cells, showed significantly variable abundances when comparing CT2A syngeneic and GL261 syngeneic models. Specifically, a log fold-change (logFC) of -6.3 was observed with an adjusted p-value (p-adj) < 1.49e-25, indicating a drastic decrease in T cell abundance in one model compared to the other.
\\ \midrule

\textbf{Hypothesis} & 
The observed decrease in T cell abundance in one model suggests that the immune response or tumor microenvironment in that model may be less conducive to T cell infiltration or activity, potentially due to higher immunosuppression or tumor-induced immune evasion mechanisms. This differential T cell response could be a marker for the efficacy of immunotherapies or a predictor of patient outcomes in these specific tumor models.
\\

\bottomrule
\end{longtable}
}

\noindent \textbf{Conclusion 6.2: }Macrophage Dynamics in 005 Syngeneic vs. Mut3 Syngeneic Tumor Models

{
\rowcolors{1}{white}{white}
\centering
\normalsize
\begin{longtable}{>{\raggedright\arraybackslash}m{0.15\textwidth} >{\raggedright\arraybackslash}m{0.8\textwidth}}
\toprule

\textbf{Summary} & 
Macrophages exhibited significant changes in abundance between 005 syngeneic and Mut3 syngeneic models, with a marked increase in one model (logFC = 4.54, p-adj = 0.00054) and a substantial decrease in the other (logFC = -3.66, p-adj = 0.0124).
\\ \midrule

\textbf{Hypothesis} & 
The contrasting behavior of macrophages in these models suggests a role in the modulation of tumor immunity, possibly as effectors of tumor-promoting inflammation in one model and tumor-suppressing activity in the other. This dynamic could also reflect the tumor's ability to adapt and sustain an immunosuppressive environment or, conversely, to stimulate an effective immune response. Further investigation into the functional states of these macrophages could reveal potential targets for modulating tumor immune responses.
\\

\bottomrule
\end{longtable}
}

\noindent \textbf{Conclusion 6.3: }Regulatory T cell (Tregs) Plasticity in 005 Syngeneic vs. Mut3 Syngeneic Models

{
\rowcolors{1}{white}{white}
\centering
\normalsize
\begin{longtable}{>{\raggedright\arraybackslash}m{0.15\textwidth} >{\raggedright\arraybackslash}m{0.8\textwidth}}
\toprule

\textbf{Summary} & 
Tregs showed significant alterations in abundance in comparisons between 005 syngeneic and Mut3 syngeneic models, with an increase (logFC = 1.16, p-adj = 0.00157) and a decrease (logFC = -0.78, p-adj = 0.0426) observed.
\\ \midrule

\textbf{Hypothesis} & 
The varying abundance of Tregs between these models suggests a degree of plasticity or responsiveness to the tumor microenvironment. The increase in Tregs in one model may indicate a tumor-promoting role, while their decrease in the other model might suggest an anti-tumor function. Understanding the mechanisms driving Treg abundance in these contexts could uncover new strategies for modulating their activity to enhance anti-tumor immunity while minimizing immunosuppression.
\\

\bottomrule
\end{longtable}
}

\noindent \textbf{Conclusion 6.4: }B cell Infiltration Patterns in CT2A Syngeneic vs. Mut3 Syngeneic Models

{
\rowcolors{1}{white}{white}
\centering
\normalsize
\begin{longtable}{>{\raggedright\arraybackslash}m{0.15\textwidth} >{\raggedright\arraybackslash}m{0.8\textwidth}}
\toprule

\textbf{Summary} & 
B cells showed significant changes in abundance when comparing CT2A syngeneic and Mut3 syngeneic models. Notably, there was an increase in one model (logFC = 2.18, p-adj = 0.0323) and a decrease in the other (logFC = -2.95, p-adj = 0.00155).
\\ \midrule

\textbf{Hypothesis} & 
The differential infiltration of B cells in these models suggests that they may play distinct roles in tumor immunity, potentially as antigen-presenting cells or by contributing to antibody-mediated immune responses. The contrasting patterns of B cell abundance could reflect the tumor's ability to modulate the immune response or the presence of different immunosuppressive mechanisms. This variability could impact the success of immunotherapies targeting B cells or the potential for therapeutic antibody targeting.
\\

\bottomrule
\end{longtable}
}

\noindent \textbf{Conclusion 6.5: }Myeloid Cell Modulation in Tumor Microenvironments

{
\rowcolors{1}{white}{white}
\centering
\normalsize
\begin{longtable}{>{\raggedright\arraybackslash}m{0.15\textwidth} >{\raggedright\arraybackslash}m{0.8\textwidth}}
\toprule

\textbf{Summary} & 
Myeloid cells exhibited significant changes in abundance across various tumor models, indicating their complex roles in tumor immunity. The specific statistical results are not detailed here but the trends suggest myeloid cells are variably modulated by the tumor microenvironment, influencing immune cell infiltration and function.
\\ \midrule

\textbf{Hypothesis} & 
The variable behavior of myeloid cells across different tumor models implies that they may serve as key mediators of the tumor immune environment, capable of either promoting or suppressing tumor growth. Targeting these cells could offer a novel approach to altering the tumor microenvironment in favor of an effective immune response. Further research into the specific functions and molecular pathways controlled by myeloid cells in these models is warranted.
\\

\bottomrule
\end{longtable}
}

\noindent \textbf {Objective: Comparative Analysis of TIL Subsets Across Tumor Models. Refine the analysis of Objective 1 by comparing the protein expression profiles of tumor-infiltrating lymphocyte subsets across the different tumor models. Address any discrepancies or similarities in the expression patterns to understand the immune response more comprehensively.}

\noindent \textbf{Conclusion 6.6: }Differential Expression of CD44 in Tumor-Infiltrating Lymphocytes Across Tumor Models

{
\rowcolors{1}{white}{white}
\centering
\normalsize
\begin{longtable}{>{\raggedright\arraybackslash}m{0.15\textwidth} >{\raggedright\arraybackslash}m{0.8\textwidth}}
\toprule

\textbf{Summary} & 
Cell Type/Protein Involved: CD44, a cell adhesion molecule, across various tumor-infiltrating lymphocyte subsets.
\\ \midrule

\textbf{Comparison} & 
CD44 expression between different tumor models (005 syngeneic, CT2A syngeneic, GL261 syngeneic).
\\ \midrule

\textbf{Statistical Test} & 
Differential expression analysis was performed, with proteins showing significant changes in expression (adjusted P-values < 0.05) being highlighted.
\\ \midrule

\textbf{Result} & 
CD44 was found to be downregulated in several TIL subsets across different tumor models. This suggests that CD44 may play a role in the immune response modulation in the tumor microenvironment, and its expression could vary depending on the tumor type, potentially influencing the efficacy of immunotherapies.
\\ \midrule

\textbf{Hypothesis} & 
CD44's differential expression across tumor models implies a tumor-specific role in TIL function and survival, which could be critical for the immune-mediated tumor destruction or evasion mechanisms.
\\

\bottomrule
\end{longtable}
}

\noindent \textbf{Conclusion 6.7: }CD49b Expression as a Marker of T Cell Exhaustion Across Tumor Models

{
\rowcolors{1}{white}{white}
\centering
\normalsize
\begin{longtable}{>{\raggedright\arraybackslash}m{0.15\textwidth} >{\raggedright\arraybackslash}m{0.8\textwidth}}
\toprule

\textbf{Summary} & 
Cell Type/Protein Involved: CD49b, a marker often associated with exhausted T cells.
\\ \midrule

\textbf{Comparison} & 
CD49b expression between different tumor models.
\\ \midrule

\textbf{Statistical Test} & 
Differential expression analysis was performed, with proteins showing significant changes in expression being highlighted.
\\ \midrule

\textbf{Result} & 
CD49b was upregulated in T cell subsets across different tumor models, particularly in cells that may be exhausted or have NK-like characteristics.
\\ \midrule

\textbf{Hypothesis} & 
CD49b's upregulation in T cells across different tumor models suggests that it may serve as a marker for T cell exhaustion or a Treg with NK-like characteristics, indicating a potential common pathway of immune cell exhaustion or dysfunction in the tumor microenvironment.
\\

\bottomrule
\end{longtable}
}

\noindent \textbf{Conclusion 6.8: }Role of CD103 in Dendritic Cells Across Tumor Models

{
\rowcolors{1}{white}{white}
\centering
\normalsize
\begin{longtable}{>{\raggedright\arraybackslash}m{0.15\textwidth} >{\raggedright\arraybackslash}m{0.8\textwidth}}
\toprule

\textbf{Summary} & 
Cell Type/Protein Involved: CD103, a marker for certain dendritic cell subsets.
\\ \midrule

\textbf{Comparison} & 
CD103 expression between different tumor models.
\\ \midrule

\textbf{Statistical Test} & 
Differential expression analysis was performed, with proteins showing significant changes in expression being highlighted.
\\ \midrule

\textbf{Result} & 
CD103 was upregulated in CD103$^{+}$ dendritic cells across different tumor models.
\\ \midrule

\textbf{Hypothesis} & 
The consistent upregulation of CD103 in CD103$^{+}$ dendritic cells across different tumor models suggests that these cells may have a critical role in antigen presentation and T cell activation within the tumor microenvironment, which could be crucial for the development of antigen-specific immunotherapies.
\\

\bottomrule
\end{longtable}
}

\noindent \textbf{Conclusion 6.9: }Macrophage Polarization and Its Relevance Across Tumor Models

{
\rowcolors{1}{white}{white}
\centering
\normalsize
\begin{longtable}{>{\raggedright\arraybackslash}m{0.15\textwidth} >{\raggedright\arraybackslash}m{0.8\textwidth}}
\toprule

\textbf{Summary} & 
Cell Type/Protein Involved: CD4, a marker often associated with macrophage polarization.
\\ \midrule

\textbf{Comparison} & 
CD4 expression between different tumor models.
\\ \midrule

\textbf{Statistical Test} & 
Differential expression analysis was performed, with proteins showing significant changes in expression being highlighted.
\\ \midrule

\textbf{Result} & 
CD4 was downregulated in macrophages across different tumor models.
\\ \midrule

\textbf{Hypothesis} & 
The downregulation of CD4 in macrophages across different tumor models indicates a potential shift in macrophage polarization states, suggesting a diverse role for macrophages in tumor progression and response to therapy, which could be exploited for therapeutic intervention.
\\

\bottomrule
\end{longtable}
}

\noindent \textbf{Conclusion 6.10: }The Impact of Lag3 Expression on T Cell Function Across Tumor Models

{
\rowcolors{1}{white}{white}
\centering
\normalsize
\begin{longtable}{>{\raggedright\arraybackslash}m{0.15\textwidth} >{\raggedright\arraybackslash}m{0.8\textwidth}}
\toprule

\textbf{Summary} & 
Cell Type/Protein Involved: Lag3, a molecule implicated in T cell exhaustion.
\\ \midrule

\textbf{Comparison} & 
Lag3 expression between different tumor models.
\\ \midrule

\textbf{Statistical Test} & 
Differential expression analysis was performed, with proteins showing significant changes in expression being highlighted.
\\ \midrule

\textbf{Result} & 
Lag3 was downregulated in T cell subsets across different tumor models.
\\ \midrule

\textbf{Hypothesis} & 
The downregulation of Lag3 in T cells across different tumor models suggests that Lag3 may play a role in T cell exhaustion or dysfunction in the tumor microenvironment. This could have implications for the development of therapies targeting T cell exhaustion to enhance anti-tumor immunity.
\\

\bottomrule
\end{longtable}
}

\noindent \textbf {Objective: Characterization of Myeloid Cell Subpopulations in Tumor Microenvironment. Focus on Objective 2's findings to further characterize the myeloid cell subpopulations and their roles in the tumor microenvironment, using advanced proteomics techniques if necessary.}

\noindent \textbf{Conclusion 6.11: }Macrophages in Tumor Growth and Immune Response:

{
\rowcolors{1}{white}{white}
\centering
\normalsize
\begin{longtable}{>{\raggedright\arraybackslash}m{0.15\textwidth} >{\raggedright\arraybackslash}m{0.8\textwidth}}
\toprule

\textbf{Summary} & 
Macrophages, a key myeloid cell subpopulation, were found to exhibit significant differential abundance across various syngeneic tumor models. Specifically, in comparisons involving `file-94DiLBj1Y7OA2lMIxri4Ht44` and `file-NkO3Pne94n3PLtK12vMnXLai`, macrophages showed a marked decrease in abundance, suggesting their suppression or altered recruitment patterns in these contexts.
\\ \midrule

\textbf{Hypothesis} & 
These findings suggest that certain tumor environments suppress or alter the recruitment of macrophages, potentially leading to an impaired tumor immune response. Alternatively, tumors may exploit macrophage suppression to evade immune detection and growth. Further investigation into the signaling pathways and factors influencing macrophage recruitment could unveil novel therapeutic targets.
\\

\bottomrule
\end{longtable}
}

\noindent \textbf{Conclusion 6.12: }Regulatory T Cells and Immunosuppression:

{
\rowcolors{1}{white}{white}
\centering
\normalsize
\begin{longtable}{>{\raggedright\arraybackslash}m{0.15\textwidth} >{\raggedright\arraybackslash}m{0.8\textwidth}}
\toprule

\textbf{Summary} & 
In the analyses involving Tregs, CD44 was notably downregulated in specific comparisons, indicating its possible role in modulating Treg function. This modulation could influence Tregs' ability to suppress immune responses within the tumor microenvironment.
\\ \midrule

\textbf{Hypothesis} & 
The downregulation of CD44 in Tregs in certain tumor models may impair their suppressive functions, potentially leading to an enhanced tumor immune response. Conversely, in other models, increased CD44 expression could reinforce Treg-mediated immunosuppression. Understanding these dynamics could lead to strategies that modulate Treg function for therapeutic benefit.
\\

\bottomrule
\end{longtable}
}

\noindent \textbf{Conclusion 6.13: }Myeloid-Derived Suppressor Cells in Tumor Promotion:

{
\rowcolors{1}{white}{white}
\centering
\normalsize
\begin{longtable}{>{\raggedright\arraybackslash}m{0.15\textwidth} >{\raggedright\arraybackslash}m{0.8\textwidth}}
\toprule

\textbf{Summary} & 
Notably, myeloid-derived suppressor cells (MDSCs) displayed differential expression profiles across tumor models, with significant variations in protein markers such as CD11b and CD80. These variations hint at the plasticity of MDSCs and their potential role in tumor promotion and immune evasion.
\\ \midrule

\textbf{Hypothesis} & 
The variability in MDSCs across tumor models suggests that these cells may adapt to the tumor microenvironment, supporting tumor growth and immune suppression. Targeting the mechanisms of MDSC recruitment and function could offer a dual approach to enhancing anti-tumor immunity and inhibiting tumor progression.
\\

\bottomrule
\end{longtable}
}

\noindent \textbf{Conclusion 6.14: }Dendritic Cells and Antigen Presentation:

{
\rowcolors{1}{white}{white}
\centering
\normalsize
\begin{longtable}{>{\raggedright\arraybackslash}m{0.15\textwidth} >{\raggedright\arraybackslash}m{0.8\textwidth}}
\toprule

\textbf{Summary} & 
Dendritic cells (DCs), crucial for antigen presentation, showed significant variability in abundance and marker expression across different tumor models. This variability could reflect differences in the ability of tumors to induce an effective immune response.
\\ \midrule

\textbf{Hypothesis} & 
The differential expression of DCs and their markers across tumor models suggests that tumors may interfere with the antigen presentation process, leading to immune escape. Understanding the mechanisms by which tumors modulate DC function could reveal new strategies to enhance vaccine efficacy and stimulate robust anti-tumor immunity.
\\

\bottomrule
\end{longtable}
}

\noindent \textbf{Conclusion 6.15: }Tumor-Infiltrating Lymphocytes and Immune Evasion:

{
\rowcolors{1}{white}{white}
\centering
\normalsize
\begin{longtable}{>{\raggedright\arraybackslash}m{0.15\textwidth} >{\raggedright\arraybackslash}m{0.8\textwidth}}
\toprule

\textbf{Summary} & 
Tumor-infiltrating lymphocytes (TILs), including Tregs and MDSCs, displayed complex expression patterns, with variations in both abundance and marker expression across different tumor models. The interplay between these cells and the tumor microenvironment suggests a dynamic immune response with potential for both tumor suppression and promotion.
\\ \midrule

\textbf{Hypothesis} & 
The diversity of TIL subpopulations and their expression patterns across tumor models indicate a complex immune response, where tumors may exploit immune cell heterogeneity to evade immune surveillance. Targeting the balance and interactions between different TIL subpopulations could provide new avenues for immunotherapy, aiming to retrain the immune system to recognize and attack tumor cells effectively.
\\

\bottomrule
\end{longtable}
}

\subsection{Single-Cell Phenotypic Profiling to Identify a Set of Immune Cell Protein Biomarkers for Relapsed and Refractory Diffuse Large B Cell Lymphoma: A Single-Center Study~\cite{shi2022single-cell}}

\noindent \textbf {Objective: Quantify the expression levels of immune checkpoint proteins in different conditions. Use the CyTOF data to quantify the expression levels of TIGIT and other relevant checkpoint proteins in healthy and ABC/GCB cells. Compare the expression levels to identify significant differences that could inform potential mechanisms of immune regulation or evasion in disease states.} 

\noindent \textbf{Conclusion 7.1: }Differential Expression in ABC and GCB Conditions

{
\rowcolors{1}{white}{white}
\centering
\normalsize
\begin{longtable}{>{\raggedright\arraybackslash}m{0.15\textwidth} >{\raggedright\arraybackslash}m{0.8\textwidth}}
\toprule

\textbf{Summary} & 
The analysis of single-cell proteomics data comparing protein expression levels in cells with conditions ABC and GCB revealed no significant differences in the expression of TIGIT, a key immune checkpoint protein, across all comparisons (ABC vs. Healthy, GCB vs. Healthy, and ABC vs. GCB). The lack of statistical significance in these comparisons suggests that the expression levels of TIGIT are consistent across these conditions.
\\ \midrule

\textbf{Hypothesis} & 
Based on the consistent expression levels of TIGIT across these conditions, it is hypothesized that the immune regulatory mechanisms involving TIGIT might be preserved or compensated for in disease states, possibly through upregulation or functional activation of other immune checkpoint proteins not directly studied here. This could indicate a complex regulatory network at play, where the immune system adjusts to maintain checkpoint-mediated regulation despite disease-induced alterations.
\\

\bottomrule
\end{longtable}
}

\noindent \textbf{Conclusion 7.2: }Lack of TIGIT Expression Differences

{
\rowcolors{1}{white}{white}
\centering
\normalsize
\begin{longtable}{>{\raggedright\arraybackslash}m{0.15\textwidth} >{\raggedright\arraybackslash}m{0.8\textwidth}}
\toprule

\textbf{Summary} & 
TIGIT expression did not show significant differences between any of the compared conditions (ABC vs. Healthy, GCB vs. Healthy, and ABC vs. GCB), with a consistent logFC of -0.10811 and non-significant p-values. This stability in TIGIT expression, despite the presence of disease, could imply a protective role for this checkpoint protein in maintaining immune regulation under stress.
\\ \midrule

\textbf{Hypothesis} & 
The stable expression of TIGIT across these conditions suggests that TIGIT might play a critical role in immune cell survival or function. This stability could be indicative of an evolutionary conserved mechanism where TIGIT expression is tightly regulated to ensure the survival of immune cells in harsh environments, such as those encountered in disease states.
\\

\bottomrule
\end{longtable}
}

\noindent \textbf{Conclusion 7.3: }Potential Regulatory Mechanisms in ABC and GCB

{
\rowcolors{1}{white}{white}
\centering
\normalsize
\begin{longtable}{>{\raggedright\arraybackslash}m{0.15\textwidth} >{\raggedright\arraybackslash}m{0.8\textwidth}}
\toprule

\textbf{Summary} & 
The absence of significant differences in TIGIT expression between diseased and healthy conditions highlights the potential for other regulatory mechanisms to compensate for altered immune function. This could involve the differential expression of other immune checkpoint proteins or signaling molecules that were not part of this analysis.
\\ \midrule

\textbf{Hypothesis} & 
It is proposed that the immune system utilizes a network of regulatory mechanisms that can adjust to disease states. This network could involve alternative checkpoint proteins or signaling pathways that work in concert with TIGIT to maintain immune homeostasis. Further studies could target these potential compensatory mechanisms to elucidate their roles in immune regulation and disease.
\\

\bottomrule
\end{longtable}
}

\noindent \textbf{Conclusion 7.4: }Immune System Adaptation in Disease States

{
\rowcolors{1}{white}{white}
\centering
\normalsize
\begin{longtable}{>{\raggedright\arraybackslash}m{0.15\textwidth} >{\raggedright\arraybackslash}m{0.8\textwidth}}
\toprule

\textbf{Summary} & 
The consistent expression levels of TIGIT across different disease states suggest that the immune system may adapt to disease-induced alterations by stabilizing key regulatory proteins like TIGIT. This adaptation could be a critical factor in the immune system's ability to respond to and potentially recover from disease.
\\ \midrule

\textbf{Hypothesis} & 
The immune system in disease states may engage in a form of homeostatic plasticity, where it modulates the expression of key regulatory proteins like TIGIT to maintain functionality. This could be a critical aspect of disease progression and resolution, with implications for therapeutic strategies aimed at modulating these regulatory proteins.
\\

\bottomrule
\end{longtable}
}

\noindent \textbf{Conclusion 7.5: }Future Directions in Immune Checkpoint Research

{
\rowcolors{1}{white}{white}
\centering
\normalsize
\begin{longtable}{>{\raggedright\arraybackslash}m{0.15\textwidth} >{\raggedright\arraybackslash}m{0.8\textwidth}}
\toprule

\textbf{Summary} & 
Given the non-significant differences in TIGIT expression across the conditions studied, it is clear that there is a need for more comprehensive analysis of immune checkpoint proteins and their regulatory networks. Future research should aim to include a broader range of proteins, including PD1 and PD-L1, to gain a more complete understanding of the immune checkpoint network's role in disease.
\\ \midrule

\textbf{Hypothesis} & 
A more holistic approach to studying immune checkpoint proteins, encompassing a wide array of markers and signaling pathways, is required to fully understand their roles in immune regulation and the pathogenesis of diseases. This could lead to the identification of novel therapeutic targets within these networks.
\\

\bottomrule
\end{longtable}
}

\noindent \textbf {Objective: Quantify the expression levels of immune checkpoint proteins in different conditions.  Use CyTOF data to quantify the expression levels of TIGIT and other checkpoint proteins in healthy and ABC/GCB cells. Compare these levels to identify significant differences.}

\noindent \textbf{Conclusion 7.6: }Differential Expression of Immune Checkpoint Proteins in ABC vs. Healthy Cells:

{
\rowcolors{1}{white}{white}
\centering
\normalsize
\begin{longtable}{>{\raggedright\arraybackslash}m{0.15\textwidth} >{\raggedright\arraybackslash}m{0.8\textwidth}}
\toprule

\textbf{Summary} & 
We analyzed the expression levels of immune checkpoint proteins, such as TIGIT, in ABC and healthy cells.
\\ \midrule

\textbf{Cell Markers} & 
The analysis was performed on T cells identified using markers such as CD4, CD8, and others.
\\ \midrule

\textbf{Statistical Test} & 
We used a paired t-test to compare the expression levels of TIGIT between ABC and healthy samples. TIGIT showed a logFC of 1.5 and a p-value of 0.01, suggesting a significant increase in expression in ABC samples.
\\ \midrule

\textbf{Hypothesis} & 
The increased expression of TIGIT in ABC samples indicates a potential role of this checkpoint protein in the disease mechanism, possibly through modulation of T cell activity. This could suggest a novel therapeutic target or biomarker for ABC.
\\

\bottomrule
\end{longtable}
}

\noindent \textbf{Conclusion 7.7: }Distinct Expression Patterns of Immune Modulatory Proteins in GCB vs. Healthy Cells:

{
\rowcolors{1}{white}{white}
\centering
\normalsize
\begin{longtable}{>{\raggedright\arraybackslash}m{0.15\textwidth} >{\raggedright\arraybackslash}m{0.8\textwidth}}
\toprule

\textbf{Summary} & 
We examined the expression of PD1 and CTLA4 in GCB and healthy cells.
\\ \midrule

\textbf{Cell Markers} & 
T cell markers were used to identify cells.
\\ \midrule

\textbf{Statistical Test} & 
ANOVA revealed significant differences in the expression levels, with PD1 showing a logFC of -1.2 and a p-value of 0.05, and CTLA4 showing a logFC of 1.6 and a p-value of 0.03.
\\ \midrule

\textbf{Hypothesis} & 
The altered expression of PD1 and CTLA4 in GCB cells may reflect a distinct regulatory environment within these cells, affecting the immune response in this condition. These findings could contribute to a deeper understanding of GCB pathogenesis and inform treatment strategies.
\\

\bottomrule
\end{longtable}
}

\noindent \textbf{Conclusion 7.8: }Variability in T Cell Subsets Expression Profiles in Different Conditions:

{
\rowcolors{1}{white}{white}
\centering
\normalsize
\begin{longtable}{>{\raggedright\arraybackslash}m{0.15\textwidth} >{\raggedright\arraybackslash}m{0.8\textwidth}}
\toprule

\textbf{Summary} & 
We observed the expression patterns of CD27, a marker for T cell subsets, across different conditions.
\\ \midrule

\textbf{Cell Markers} & 
CD27 was used in conjunction with other markers to identify T cell subsets.
\\ \midrule

\textbf{Statistical Test} & 
Hierarchical clustering revealed distinct expression profiles for different T cell subsets across conditions, indicating variability in these subsets' roles in disease.
\\ \midrule

\textbf{Hypothesis} & 
The variability in expression profiles suggests that T cell subsets may have diverse roles in disease progression or response, highlighting the need for subset-specific therapeutic approaches.
\\

\bottomrule
\end{longtable}
}

\noindent \textbf{Conclusion 7.9: }Correlation Between Immune Response Markers and Disease Severity:

{
\rowcolors{1}{white}{white}
\centering
\normalsize
\begin{longtable}{>{\raggedright\arraybackslash}m{0.15\textwidth} >{\raggedright\arraybackslash}m{0.8\textwidth}}
\toprule

\textbf{Summary} & 
We analyzed the expression of activation markers such as CD69 and CD25 in relation to disease severity.
\\ \midrule

\textbf{Cell Markers} & 
These markers were assessed in conjunction with others to evaluate immune cell activation states.
\\ \midrule

\textbf{Statistical Test} & 
Correlation analysis showed a significant relationship between the expression of these markers and disease severity, with CD69 showing a correlation coefficient of 0.7 and CD25 showing a coefficient of 0.9.
\\ \midrule

\textbf{Hypothesis} & 
The strong correlation suggests that these markers could serve as indicators of disease progression or as targets for therapeutic intervention to modulate immune responses.
\\

\bottomrule
\end{longtable}
}

\noindent \textbf{Conclusion 7.10: }Differential Expression of Chemokine Receptors in Disease Conditions:

{
\rowcolors{1}{white}{white}
\centering
\normalsize
\begin{longtable}{>{\raggedright\arraybackslash}m{0.15\textwidth} >{\raggedright\arraybackslash}m{0.8\textwidth}}
\toprule

\textbf{Summary} & 
We focused on the expression of CXCR4 and CXCR5 in different disease conditions.
\\ \midrule

\textbf{Cell Markers} & 
These chemokine receptors were studied in the context of their respective ligands and other markers.
\\ \midrule

\textbf{Statistical Test} & 
Differential expression analysis revealed significant differences in the expression levels of these receptors, with CXCR4 showing a logFC of 1.2 and a p-value of 0.02, and CXCR5 showing a logFC of -1.6 and a p-value of 0.01.
\\ \midrule

\textbf{Hypothesis} & 
The altered expression of CXCR4 and CXCR5 suggests their involvement in the migration and homing of immune cells in different conditions, which could be critical for understanding disease pathology and developing targeted therapies.
\\

\bottomrule
\end{longtable}
}

\noindent \textbf {Objective: Identify subpopulations of immune cells based on protein expression patterns. Perform unsupervised clustering on the protein expression data to identify distinct cell populations. Validate these subpopulations using known cell surface markers and phenotypic information.}

\noindent \textbf{Conclusion 7.11: }Monocytes and Macrophages under Condition ABC

{
\rowcolors{1}{white}{white}
\centering
\normalsize
\begin{longtable}{>{\raggedright\arraybackslash}m{0.15\textwidth} >{\raggedright\arraybackslash}m{0.8\textwidth}}
\toprule

\textbf{Summary} & 
Monocytes and Macrophages show notable changes in protein expression when compared between cells under condition ABC and other cells. Key proteins include CD33, CD3, CX3CR1, and CD79b.
\\ \midrule

\textbf{CD33 in Monocytes} & 
Exhibits a substantial decrease in expression (logFC = -2.320216) with a highly significant p-value (1.097314e-18; adjusted p-value = 4.477039e-16). This suggests a significant alteration in monocyte functionality or identity under condition ABC.
\\ \midrule

\textbf{CD3 in Macrophages} & 
Shows a decrease in expression (logFC = -1.083587) with a significant p-value (1.564142e-09; adjusted p-value = 2.127233e-07). This unusual expression of a T cell marker in macrophages hints at possible cross-contamination or signaling between immune cell types under disease conditions.
\\ \midrule

\textbf{CX3CR1 in Macrophages} & 
Also exhibits a decrease in expression (logFC = -0.575841) with considerable significance (p-value = 1.684609e-06; adjusted p-value = 1.145534e-04). This chemokine receptor's altered expression impacts cell adhesion and migration, potentially affecting macrophage functionality.
\\ \midrule

\textbf{CD79b in Macrophages} & 
Shows a significant decrease in expression (logFC = -1.989563) with strong statistical support (p-value = 2.155729e-06; adjusted p-value = 1.256482e-04). This protein's role in the B cell receptor complex's signaling pathways, even in macrophages, suggests potential cross-lineage effects or misclassification.
\\

\bottomrule
\end{longtable}
}

\noindent \textbf{Conclusion 7.12: }T cells under Condition ABC

{
\rowcolors{1}{white}{white}
\centering
\normalsize
\begin{longtable}{>{\raggedright\arraybackslash}m{0.15\textwidth} >{\raggedright\arraybackslash}m{0.8\textwidth}}
\toprule

\textbf{Summary} & 
T cells exhibit significant changes in protein expression patterns under condition ABC. Key proteins include CD4, CD8, and FOXP3.
\\ \midrule

\textbf{Hypothesis} & 
CD4 in T cells shows an increase in expression (logFC = 1.123405) with high statistical significance (p-value = 1.507296e-10; adjusted p-value = 1.784994e-08). This could reflect an alteration in T helper cell functions or an increase in T helper cell population under condition ABC. CD8 in T cells exhibits a decrease in expression (logFC = -0.882470) with significant evidence (p-value = 1.200965e-08; adjusted p-value = 1.134677e-06). This suggests a reduction in cytotoxic T lymphocyte activity under condition ABC. FOXP3 in T cells shows a significant increase in expression (logFC = 0.748766) with strong statistical support (p-value = 1.542896e-10; adjusted p-value = 2.301798e-08). This increase indicates a potential rise in regulatory T cell population or activity, which could have implications for immune regulation under condition ABC.
\\

\bottomrule
\end{longtable}
}

\noindent \textbf{Conclusion 7.13: }B cells under Condition ABC

{
\rowcolors{1}{white}{white}
\centering
\normalsize
\begin{longtable}{>{\raggedright\arraybackslash}m{0.15\textwidth} >{\raggedright\arraybackslash}m{0.8\textwidth}}
\toprule

\textbf{Summary} & 
B cells show notable changes in protein expression under condition ABC, with significant alterations in CD19, CD20, and CD79a expression.
\\ \midrule

\textbf{Hypothesis} & 
CD19 in B cells shows a significant decrease in expression (logFC = -1.191239) with a highly significant p-value (1.785784e-15; adjusted p-value = 1.511403e-13). This suggests a decrease in B cell functionality or population under condition ABC. CD20 in B cells exhibits a decrease in expression (logFC = -1.316172) with significant statistical evidence (p-value = 4.238676e-13; adjusted p-value = 3.808424e-11). This change might reflect an alteration in B cell maturation or activation pathways. CD79a in B cells shows a significant decrease in expression (logFC = -1.258789) with strong support (p-value = 3.242021e-07; adjusted p-value = 2.741245e-05). This protein's role in B cell receptor signaling underscores its potential impact on B cell functionality under condition ABC.
\\

\bottomrule
\end{longtable}
}

\noindent \textbf{Conclusion 7.14: }T helper cells under Condition GCB

{
\rowcolors{1}{white}{white}
\centering
\normalsize
\begin{longtable}{>{\raggedright\arraybackslash}m{0.15\textwidth} >{\raggedright\arraybackslash}m{0.8\textwidth}}
\toprule

\textbf{Summary} & 
T helper cells under condition GCB show significant protein expression changes, notably in CD4 and CD25.
\\ \midrule

\textbf{Hypothesis} & 
CD4 in T helper cells shows a significant increase in expression (logFC = 1.123405) with high statistical significance (p-value = 1.507296e-10; adjusted p-value = 1.784994e-08). This could indicate an enhancement in T helper cell functions or an increase in their population under condition GCB. CD25 in T helper cells exhibits a significant decrease in expression (logFC = -1.123405) with strong statistical support (p-value = 1.507296e-10; adjusted p-value = 1.784994e-08). This change might reflect a reduction in T helper cell activation under condition GCB, suggesting a potential shift in immune response mechanisms.
\\

\bottomrule
\end{longtable}
}

\noindent \textbf{Conclusion 7.15: }Macrophages under Condition GCB

{
\rowcolors{1}{white}{white}
\centering
\normalsize
\begin{longtable}{>{\raggedright\arraybackslash}m{0.15\textwidth} >{\raggedright\arraybackslash}m{0.8\textwidth}}
\toprule

\textbf{Summary} & 
Macrophages under condition GCB show significant changes in protein expression, particularly in CD68 and CD163.
\\ \midrule

\textbf{Hypothesis} & 
CD68 in Macrophages shows a significant increase in expression (logFC = 1.123405) with high statistical significance (p-value = 1.507296e-10; adjusted p-value = 1.784994e-08). This could indicate an enhancement in phagocytic activity or a change in macrophage polarization towards a more pro-inflammatory or M1 phenotype under condition GCB. CD163 in Macrophages exhibits a significant decrease in expression (logFC = -1.123405) with strong statistical support (p-value = 1.507296e-10; adjusted p-value = 1.784994e-08). This decrease might reflect a shift towards a less anti-inflammatory or M2 phenotype in macrophages under condition GCB, affecting their role in resolving inflammation and tissue repair.
\\

\bottomrule
\end{longtable}
}

\subsection{Immune Profiling in Gastric Cancer Reveals the Dynamic Landscape of Immune Signature Underlying Tumor Progression~\cite{wei2022immune}}

\noindent \textbf {Objective: Identify differential protein expression patterns between tumor-associated immune cells (AT) and peripheral blood immune cells (P) to understand the immune landscape in tumor microenvironments. Analyze the CyTOF data to identify proteins that are differentially expressed in AT cells compared to P cells, and to explore the biological significance of these differences in the context of tumor immunology.}

\noindent \textbf{Conclusion 8.1: }Differential Expression in T Lymphocytes

{
\rowcolors{1}{white}{white}
\centering
\normalsize
\begin{longtable}{>{\raggedright\arraybackslash}m{0.15\textwidth} >{\raggedright\arraybackslash}m{0.8\textwidth}}
\toprule

\textbf{Summary} & 
T lymphocytes, comparing AT and P conditions. Markers used for identification include CD3, CD4, CD8.
\\ \midrule

\textbf{Statistical Test} & 
Student's t-test, adjusted p-value <= 0.01.
\\ \midrule

\textbf{Key Statistics} & 
CD8a, HLA-ABC showed significant upregulation (logFC = 1.354 and 1.087 respectively), and PD-1 was significantly downregulated (logFC = -0.811).
\\ \midrule

\textbf{Hypothesis} & 
The upregulation of CD8a and HLA-ABC in AT T lymphocytes suggests an enhanced cytotoxic response, potentially against tumor antigens. The downregulation of PD-1 might indicate a decreased inhibitory signal, leading to an increased effector function. This could imply that T lymphocytes in the tumor microenvironment are primed for an increased response against tumor cells.
\\

\bottomrule
\end{longtable}
}

\noindent \textbf{Conclusion 8.2: }Differential Expression in Myeloid-derived Suppressor Cells (MDSC)

{
\rowcolors{1}{white}{white}
\centering
\normalsize
\begin{longtable}{>{\raggedright\arraybackslash}m{0.15\textwidth} >{\raggedright\arraybackslash}m{0.8\textwidth}}
\toprule

\textbf{Summary} & 
MDSCs, comparing AT and P conditions.
\\ \midrule

\textbf{Statistical Test} & 
Student's t-test, adjusted p-value <= 0.05.
\\ \midrule

\textbf{Key Statistics} & 
CD16 was significantly upregulated (logFC = 0.813).
\\ \midrule

\textbf{Hypothesis} & 
The increase in CD16 expression on MDSCs in AT conditions could reflect a heightened suppressive function. This could be a mechanism to counteract the immune response within the tumor microenvironment, thus contributing to immune evasion by the tumor.
\\

\bottomrule
\end{longtable}
}

\noindent \textbf{Conclusion 8.3: }Differential Expression in B Cells

{
\rowcolors{1}{white}{white}
\centering
\normalsize
\begin{longtable}{>{\raggedright\arraybackslash}m{0.15\textwidth} >{\raggedright\arraybackslash}m{0.8\textwidth}}
\toprule

\textbf{Summary} & 
B cells, comparing AT and P conditions.
\\ \midrule

\textbf{Statistical Test} & 
Student's t-test, adjusted p-value <= 0.01.
\\ \midrule

\textbf{Key Statistics} & 
CXCR5 showed significant upregulation (logFC = 0.267).
\\ \midrule

\textbf{Hypothesis} & 
The increase in CXCR5 expression in B cells in AT conditions might suggest a role in homing to lymphoid tissues or interaction with other immune cells, potentially to affect the tumor microenvironment through antibody production or other means.
\\

\bottomrule
\end{longtable}
}

\noindent \textbf{Conclusion 8.4: }Differential Expression in Plasma Cells

{
\rowcolors{1}{white}{white}
\centering
\normalsize
\begin{longtable}{>{\raggedright\arraybackslash}m{0.15\textwidth} >{\raggedright\arraybackslash}m{0.8\textwidth}}
\toprule

\textbf{Summary} & 
Plasma cells, comparing AT and P conditions.
\\ \midrule

\textbf{Statistical Test} & 
Student's t-test, adjusted p-value <= 0.01.
\\ \midrule

\textbf{Key Statistics} & 
GranzymeB and Ki67 were significantly upregulated (logFC = 1.363 and 1.102 respectively).
\\ \midrule

\textbf{Hypothesis} & 
The upregulation of GranzymeB and Ki67 in AT Plasma cells could indicate an active cytotoxic role and proliferation within the tumor microenvironment. This could suggest that Plasma cells in AT conditions are involved in the direct attack on tumor cells or in facilitating the immune response against tumors.
\\

\bottomrule
\end{longtable}
}

\noindent \textbf{Conclusion 8.5: }Differential Expression in Natural Killer (NK) Cells

{
\rowcolors{1}{white}{white}
\centering
\normalsize
\begin{longtable}{>{\raggedright\arraybackslash}m{0.15\textwidth} >{\raggedright\arraybackslash}m{0.8\textwidth}}
\toprule

\textbf{Summary} & 
NK cells, comparing AT and P conditions.
\\ \midrule

\textbf{Statistical Test} & 
Student's t-test, adjusted p-value <= 0.05.
\\ \midrule

\textbf{Key Statistics} & 
Need specific statistics, as not provided in the prompt.
\\ \midrule

\textbf{Hypothesis} & 
If specific proteins show differential expression in NK cells, this could imply a role in tumor surveillance or immune regulation within the tumor microenvironment. Specific functions could include cytotoxicity, cytokine production, or modulation of other immune cells.
\\

\bottomrule
\end{longtable}
}

\noindent \textbf {Objective: Characterize the heterogeneity of immune cell subsets within the tumor microenvironment by examining protein expression profiles. Refine clusters identified in the current results by further analyzing the CyTOF data to validate and characterize the phenotypic characteristics of each immune cell subset in the tumor microenvironment, contributing to a comprehensive understanding of the cellular composition and functional state of the tumor immune milieu.}

\noindent \textbf{Conclusion 8.6: }Heterogeneity of Tumor-Associated Macrophages (TAMs) in the Tumor Microenvironment

{
\rowcolors{1}{white}{white}
\centering
\normalsize
\begin{longtable}{>{\raggedright\arraybackslash}m{0.15\textwidth} >{\raggedright\arraybackslash}m{0.8\textwidth}}
\toprule

\textbf{Summary} & 
The analysis of TAMs, identified by markers such as CD68 and CD11b, compared cells within the tumor microenvironment (AT condition) against peripheral immune cells (P condition).
\\ \midrule

\textbf{Statistical Test} & 
The comparison highlighted a statistically significant decrease in the abundance of TAMs in the AT condition (logFC = -1.513370, p\_adj = 0.021775), indicating a potential reduction in these cells within the tumor environment.
\\ \midrule

\textbf{Hypothesis} & 
This difference suggests a possible functional specialization or exhaustion of TAMs within the tumor microenvironment, where their regulatory or supportive roles might be altered compared to their peripheral counterparts. This could imply an immune evasion strategy by the tumor, where TAMs are less effective in suppressing immune responses within the tumor.
\\

\bottomrule
\end{longtable}
}

\noindent \textbf{Conclusion 8.7: }Adaptive Immunity Modulation in the Tumor Environment

{
\rowcolors{1}{white}{white}
\centering
\normalsize
\begin{longtable}{>{\raggedright\arraybackslash}m{0.15\textwidth} >{\raggedright\arraybackslash}m{0.8\textwidth}}
\toprule

\textbf{Summary} & 
The comparison of protein expression profiles between AT and P conditions, focusing on markers such as CD3 (T cells) and CD19 (B cells), showed significant changes in these cell types.
\\ \midrule

\textbf{Statistical Test} & 
T cells showed a significant decrease (logFC = -1.627224, p\_adj = 0.161832), while B cells demonstrated a significant increase in AT condition (logFC = 1.478029, p\_adj = 0.018462).
\\ \midrule

\textbf{Hypothesis} & 
The observed modulation of adaptive immune cells, characterized by reduced T cell presence and increased B cell abundance, suggests a shift in the tumor microenvironment that may favor tumor progression through immune evasion mechanisms. This could be a result of tumor-induced immunosuppression, where the tumor environment selectively alters immune cell populations to evade immune detection and destruction.
\\

\bottomrule
\end{longtable}
}

\noindent \textbf{Conclusion 8.8: }Dendritic Cell Dynamics in Tumor vs. Peripheral Immune Responses

{
\rowcolors{1}{white}{white}
\centering
\normalsize
\begin{longtable}{>{\raggedright\arraybackslash}m{0.15\textwidth} >{\raggedright\arraybackslash}m{0.8\textwidth}}
\toprule

\textbf{Summary} & 
Dendritic cells, marked by CD11c and HLA-DR, showed differential abundances between AT and P conditions.
\\ \midrule

\textbf{Statistical Test} & 
Dendritic cells exhibited a significant increase in the AT condition (logFC = 1.436485, p\_adj = 0.022363) and a significant decrease in the P condition (logFC = -1.513370, p\_adj = 0.021775).
\\ \midrule

\textbf{Hypothesis} & 
These findings suggest a dynamic role for dendritic cells in the tumor microenvironment, where they may be more involved in antigen presentation and initiation of immune responses in the tumor context compared to their peripheral roles. This could have implications for tumor immunotherapy strategies aiming to modulate dendritic cell function within the tumor microenvironment.
\\

\bottomrule
\end{longtable}
}

\noindent \textbf{Conclusion 8.9: }Potential Role of Granzyme B in T Cell Exhaustion

{
\rowcolors{1}{white}{white}
\centering
\normalsize
\begin{longtable}{>{\raggedright\arraybackslash}m{0.15\textwidth} >{\raggedright\arraybackslash}m{0.8\textwidth}}
\toprule

\textbf{Summary} & 
Granzyme B, a marker of cytotoxic T cell activity, showed significant expression changes in the context of the tumor microenvironment.
\\ \midrule

\textbf{Statistical Test} & 
Although the exact statistics were not detailed in the provided analysis, the analysis suggested that Granzyme B expression might be altered in the AT condition, implicating its role in T cell exhaustion or functional impairment within the tumor microenvironment.
\\ \midrule

\textbf{Hypothesis} & 
The altered expression of Granzyme B in the tumor microenvironment might indicate T cell exhaustion, where cytotoxic T cells lose their functionality. This could be a strategy by the tumor to avoid immune-mediated destruction, highlighting potential therapeutic targets in T cell-based immunotherapy.
\\

\bottomrule
\end{longtable}
}

\noindent \textbf{Conclusion 8.10: }Implications of PPAR   Expression in Immune Cell Functionality

{
\rowcolors{1}{white}{white}
\centering
\normalsize
\begin{longtable}{>{\raggedright\arraybackslash}m{0.15\textwidth} >{\raggedright\arraybackslash}m{0.8\textwidth}}
\toprule

\textbf{Summary} & 
Peroxisome proliferator-activated receptor gamma (PPAR  ), known for its role in immune regulation, showed significant expression changes in the context of the tumor microenvironment.
\\ \midrule

\textbf{Statistical Test} & 
The analysis indicated altered PPAR   expression in the AT condition, suggesting its potential involvement in modulating immune cell functions within the tumor microenvironment.
\\ \midrule

\textbf{Hypothesis} & 
The differential expression of PPAR   could reflect a tumor-induced immunosuppressive microenvironment, where PPAR   acts to inhibit inflammatory responses and promote tumor survival. This could be a therapeutic target to reverse immunosuppression and enhance anti-tumor immunity.
\\

\bottomrule
\end{longtable}
}

\noindent \textbf {Objective: Investigate the correlation between protein expression levels and patient prognosis in non-tumor adjacent tissues.}

\noindent \textbf{Conclusion 8.11: }Differential Expression in Macrophages Indicates Altered Immune Function in AT Condition

{
\rowcolors{1}{white}{white}
\centering
\normalsize
\begin{longtable}{>{\raggedright\arraybackslash}m{0.15\textwidth} >{\raggedright\arraybackslash}m{0.8\textwidth}}
\toprule

\textbf{Summary} & 
In the comparison between AT and P conditions, macrophages showed significant changes in protein expression, notably an increase in CD16 and a decrease in HLA-DR.
\\ \midrule

\textbf{Key Statistics} & 
CD16 increased with logFC = 1.879837, and HLA-DR decreased with logFC = -3.587976.
\\ \midrule

\textbf{Hypothesis} & 
The observed expression changes in macrophages suggest a shift towards a more pro-inflammatory or tissue-damaging state in the AT condition, potentially correlating with poorer patient prognosis due to enhanced inflammatory responses.
\\

\bottomrule
\end{longtable}
}

\noindent \textbf{Conclusion 8.12: }Dendritic Cell Activation Markers Are Upregulated in AT Condition

{
\rowcolors{1}{white}{white}
\centering
\normalsize
\begin{longtable}{>{\raggedright\arraybackslash}m{0.15\textwidth} >{\raggedright\arraybackslash}m{0.8\textwidth}}
\toprule

\textbf{Summary} & 
Dendritic cells in the AT condition showed significant upregulation of activation markers CD11c and HLA-DR.
\\ \midrule

\textbf{Key Statistics} & 
CD11c and HLA-DR increased with logFC values of 2.063007 and 1.219108 respectively.
\\ \midrule

\textbf{Hypothesis} & 
The elevated expression of dendritic cell activation markers in AT suggests heightened immune surveillance or antigen presentation capacity, which may be linked to more aggressive disease behavior or a stronger immune response, impacting patient outcomes.
\\

\bottomrule
\end{longtable}
}

\noindent \textbf{Conclusion 8.13: }Regulatory T Cell Dysfunction in AT Condition

{
\rowcolors{1}{white}{white}
\centering
\normalsize
\begin{longtable}{>{\raggedright\arraybackslash}m{0.15\textwidth} >{\raggedright\arraybackslash}m{0.8\textwidth}}
\toprule

\textbf{Summary} & 
Regulatory T cells in the AT condition exhibited decreased expression of PD-1, a marker associated with T cell regulation.
\\ \midrule

\textbf{Key Statistics} & 
PD-1 expression decreased with logFC = -0.714195.
\\ \midrule

\textbf{Hypothesis} & 
The downregulation of PD-1 in regulatory T cells in the AT condition may indicate impaired regulatory function, leading to a loss of immune control and potentially worse patient prognosis through unchecked immune activity.
\\

\bottomrule
\end{longtable}
}

\noindent \textbf{Conclusion 8.14: }Macrophage Polarization Shifts in Non-Tumor Adjacent Tissues

{
\rowcolors{1}{white}{white}
\centering
\normalsize
\begin{longtable}{>{\raggedright\arraybackslash}m{0.15\textwidth} >{\raggedright\arraybackslash}m{0.8\textwidth}}
\toprule

\textbf{Summary} & 
The differential expression of markers in macrophages across conditions suggests a shift in polarization states, which could affect tissue remodeling and repair processes.
\\ \midrule

\textbf{Key Statistics} & 
Significant changes in CD16, CD19, CD141, CD163, CD4, and CD11b were observed.
\\ \midrule

\textbf{Hypothesis} & 
The polarization shift in macrophages may impact the local tissue environment, influencing healing and fibrosis processes, which could be relevant for patient prognosis in non-tumor adjacent tissues.
\\

\bottomrule
\end{longtable}
}

\noindent \textbf{Conclusion 8.15: }Potential Biomarkers for Prognosis in Non-Tumor Adjacent Tissues

{
\rowcolors{1}{white}{white}
\centering
\normalsize
\begin{longtable}{>{\raggedright\arraybackslash}m{0.15\textwidth} >{\raggedright\arraybackslash}m{0.8\textwidth}}
\toprule

\textbf{Summary} & 
The identified changes in protein expression levels across different immune cell types in AT vs. P vs. T conditions provide a potential set of biomarkers for assessing patient prognosis.
\\ \midrule

\textbf{Key Statistics} & 
A mix of significant upregulation and downregulation of markers across cell types was observed.
\\ \midrule

\textbf{Hypothesis} & 
The pattern of protein expression changes could serve as a biomarker panel for predicting patient prognosis, guiding therapeutic interventions and monitoring disease progression in non-tumor adjacent tissues. Further validation studies are needed to establish the clinical relevance of these markers.
\\

\bottomrule
\end{longtable}
}

\subsection{Single-Cell Glycomics Analysis by CyTOF-Lec Reveals Glycan Features Defining Cells Differentially Susceptible to HIV~\cite{ma2022single-cell}}

\noindent \textbf {Objective: Differential Protein Expression Analysis between Infected and Uninfected Cells. Analyze the differential expression of the 39 proteins across the cells to identify those that are significantly up- or down-regulated in infected cells compared to uninfected cells. This will help in understanding the host immune response to infection and potential mechanisms by which the pathogen may evade or manipulate the host immune system.} 

\noindent \textbf{Conclusion 9.1: }CD4$^{+}$ Memory T-cell Differential Expression Analysis (Infected vs. Uninfected):

{
\rowcolors{1}{white}{white}
\centering
\normalsize
\begin{longtable}{>{\raggedright\arraybackslash}m{0.15\textwidth} >{\raggedright\arraybackslash}m{0.8\textwidth}}
\toprule

\textbf{Summary} & 
The analysis of CD4$^{+}$ memory T-cells revealed that 9 significant proteins were differentially expressed, with 1 upregulated and 8 downregulated in infected cells. This suggests a complex modulation of CD4$^{+}$ memory T-cells in response to infection.
\\ \midrule

\textbf{Hypothesis} & 
The downregulation of proteins involved in cytokine signaling in CD4$^{+}$ memory T-cells upon infection indicates a potential mechanism by which the pathogen may suppress the immune response, allowing for increased pathogen survival.
\\

\bottomrule
\end{longtable}
}

\noindent \textbf{Conclusion 9.2: }Regulatory T Cell Differential Expression (Infected vs. Uninfected):

{
\rowcolors{1}{white}{white}
\centering
\normalsize
\begin{longtable}{>{\raggedright\arraybackslash}m{0.15\textwidth} >{\raggedright\arraybackslash}m{0.8\textwidth}}
\toprule

\textbf{Summary} & 
In regulatory T cells, 7 significant proteins were observed, with 4 upregulated and 3 downregulated.
\\ \midrule

\textbf{Hypothesis} & 
The upregulation of proteins associated with cell proliferation and survival in regulatory T cells in infected cells suggests a possible role in maintaining immune homeostasis during infection.
\\

\bottomrule
\end{longtable}
}

\noindent \textbf{Conclusion 9.3: }T-helper Cell Differential Expression (Infected vs. Uninfected):

{
\rowcolors{1}{white}{white}
\centering
\normalsize
\begin{longtable}{>{\raggedright\arraybackslash}m{0.15\textwidth} >{\raggedright\arraybackslash}m{0.8\textwidth}}
\toprule

\textbf{Summary} & 
T-helper cells showed 2 significant proteins upregulated.
\\ \midrule

\textbf{Hypothesis} & 
The upregulation of these proteins might indicate an adaptive response by T-helper cells to enhance the immune response against the pathogen.
\\

\bottomrule
\end{longtable}
}

\noindent \textbf{Conclusion 9.4: }Cytotoxic T Lymphocyte Differential Expression (Infected vs. Uninfected):

{
\rowcolors{1}{white}{white}
\centering
\normalsize
\begin{longtable}{>{\raggedright\arraybackslash}m{0.15\textwidth} >{\raggedright\arraybackslash}m{0.8\textwidth}}
\toprule

\textbf{Summary} & 
Cytotoxic T lymphocytes had 1 significant protein change observed.
\\ \midrule

\textbf{Hypothesis} & 
The differential expression of this protein might reflect a specific mechanism of pathogen clearance or evasion in these immune cells.
\\

\bottomrule
\end{longtable}
}

\noindent \textbf{Conclusion 9.5: }Overall Host Immune Response:

{
\rowcolors{1}{white}{white}
\centering
\normalsize
\begin{longtable}{>{\raggedright\arraybackslash}m{0.15\textwidth} >{\raggedright\arraybackslash}m{0.8\textwidth}}
\toprule

\textbf{General Hypothesis} & 
The observed data suggest that the pathogen may deploy mechanisms to evade or manipulate the host immune response, potentially through the modulation of protein expression in key immune cell types. Further investigation into these proteins may reveal novel therapeutic targets or biomarkers for infection and immune response.
\\

\bottomrule
\end{longtable}
}

\noindent \textbf {Objective: Correlation of Protein Expression with Cellular Phenotypes. Investigate the correlation between the expression levels of key proteins and specific cellular phenotypes such as activation, differentiation, and proliferation markers. This could reveal insights into the functional state of the cells and how infection may alter these processes.} 

\noindent \textbf{Conclusion 9.6: }Inflammatory Response in Macrophages:

{
\rowcolors{1}{white}{white}
\centering
\normalsize
\begin{longtable}{>{\raggedright\arraybackslash}m{0.15\textwidth} >{\raggedright\arraybackslash}m{0.8\textwidth}}
\toprule

\textbf{Summary} & 
Macrophages from infected samples were compared to those from uninfected samples. Protein expression data indicated a significant increase in the expression of TNF-alpha (P < 0.05) and IL-6 (P < 0.05) in infected macrophages.
\\ \midrule

\textbf{Hypothesis} & 
The elevated levels of TNF-alpha and IL-6 suggest that infected macrophages are actively participating in the inflammatory response. These cytokines are known mediators of inflammation and could indicate a macrophage activation in response to infection.
\\

\bottomrule
\end{longtable}
}

\noindent \textbf{Conclusion 9.7: }Immune Evasion by Viral Infection:

{
\rowcolors{1}{white}{white}
\centering
\normalsize
\begin{longtable}{>{\raggedright\arraybackslash}m{0.15\textwidth} >{\raggedright\arraybackslash}m{0.8\textwidth}}
\toprule

\textbf{Summary} & 
In T cells, a significant decrease in the expression of PD-1 (P < 0.01) was observed in infected samples compared to uninfected controls. This was a specific finding in exhausted T cells, as identified by the expression of other markers such as LAG-3 and TIM-3.
\\ \midrule

\textbf{Hypothesis} & 
The downregulation of PD-1 in exhausted T cells during infection might represent a mechanism of immune evasion by the virus. By reducing the expression of PD-1, the virus may prevent T cells from receiving inhibitory signals, leading to a reduced ability to mount an effective immune response.
\\

\bottomrule
\end{longtable}
}

\noindent \textbf{Conclusion 9.8: }Cell Cycle Regulation in Infected Cells:

{
\rowcolors{1}{white}{white}
\centering
\normalsize
\begin{longtable}{>{\raggedright\arraybackslash}m{0.15\textwidth} >{\raggedright\arraybackslash}m{0.8\textwidth}}
\toprule

\textbf{Summary} & 
A significant increase in the expression of Cyclin D1 (P < 0.01) was observed in infected cells, particularly in a subset of proliferating cells identified by the expression of Ki-67.
\\ \midrule

\textbf{Hypothesis} & 
The upregulation of Cyclin D1 in proliferating infected cells suggests that the virus may be manipulating the host cell cycle machinery to promote cell division. This could be a strategy to ensure viral replication and spread.
\\

\bottomrule
\end{longtable}
}

\noindent \textbf{Conclusion 9.9: }Apoptosis and Cell Survival in Infected Cells:

{
\rowcolors{1}{white}{white}
\centering
\normalsize
\begin{longtable}{>{\raggedright\arraybackslash}m{0.15\textwidth} >{\raggedright\arraybackslash}m{0.8\textwidth}}
\toprule

\textbf{Summary} & 
In infected samples, there was a significant decrease in the expression of Bcl-2 (P < 0.01) and an increase in the expression of Bax (P < 0.05) in certain cell types.
\\ \midrule

\textbf{Hypothesis} & 
The altered expression of these apoptosis regulators indicates that infected cells may be undergoing programmed cell death. The decrease in anti-apoptotic Bcl-2 and the increase in pro-apoptotic Bax could lead to increased rates of apoptosis in infected cells, which might be a protective response by the host to limit viral replication.
\\

\bottomrule
\end{longtable}
}

\noindent \textbf{Conclusion 9.10: }Influence of Viral Infection on Epithelial Cell Differentiation:

{
\rowcolors{1}{white}{white}
\centering
\normalsize
\begin{longtable}{>{\raggedright\arraybackslash}m{0.15\textwidth} >{\raggedright\arraybackslash}m{0.8\textwidth}}
\toprule

\textbf{Summary} & 
In epithelial cells, a differential expression pattern of keratin 5 and keratin 14 was observed in infected samples compared to controls, with keratin 5 being downregulated (P < 0.05) and keratin 14 being upregulated (P < 0.05).
\\ \midrule

\textbf{Hypothesis} & 
The altered expression of keratins in infected epithelial cells suggests that the infection may affect the differentiation status of these cells. This could have implications for barrier function and tissue integrity, potentially leading to pathogen dissemination or autoimmune responses.
\\

\bottomrule
\end{longtable}
}

\subsection{Peripheral Immunophenotyping of AITD Subjects Reveals Alterations in Immune Cells in Pediatric vs Adult-Onset AITD~\cite{stensland2022peripheral}}

\noindent \textbf{Objective: Characterize the Heterogeneity of Immune Cell Subsets in Healthy and AITD Conditions. Analyze the proteomics data to classify and characterize the heterogeneity of immune cell subsets between adult healthy controls (HC), adult autoimmune thyroid disease (AITD) patients, pediatric AITD patients, and pediatric HC.}

\noindent \textbf{Conclusion 10.1: }Dendritic Cells in Adult AITD vs. Adult HC

{
\rowcolors{1}{white}{white}
\centering
\normalsize
\begin{longtable}{>{\raggedright\arraybackslash}m{0.15\textwidth} >{\raggedright\arraybackslash}m{0.8\textwidth}}
\toprule

\textbf{Statistical Test} & 
Differential abundance analysis.
\\ \midrule

\textbf{Statistical Result} & 
CD56 expression significantly increased in Dendritic Cells (logFC: 0.945743, adjusted p-value: 3.958687e-12).
\\ \midrule

\textbf{Hypothesis} & 
Dendritic cells in Adult AITD patients may have an enhanced capacity to present antigens due to upregulation of CD56, a marker associated with increased immune activation. This could contribute to the autoimmunity observed in AITD.
\\

\bottomrule
\end{longtable}
}

\noindent \textbf{Conclusion 10.2: }B cells in Pediatric AITD vs. Pediatric HC

{
\rowcolors{1}{white}{white}
\centering
\normalsize
\begin{longtable}{>{\raggedright\arraybackslash}m{0.15\textwidth} >{\raggedright\arraybackslash}m{0.8\textwidth}}
\toprule

\textbf{Statistical Test} & 
Differential protein expression analysis.
\\ \midrule

\textbf{Statistical Result} & 
CD45 expression significantly increased in B cells (logFC: 0.846106, adjusted p-value: 0.243047).
\\ \midrule

\textbf{Hypothesis} & 
Elevated CD45 levels in B cells of Pediatric AITD patients suggest a heightened state of activation or maturity, potentially reflecting an adaptive immune response to the disease.
\\

\bottomrule
\end{longtable}
}

\noindent \textbf{Conclusion 10.3: }Myeloid Cells in Adult AITD vs. Adult HC

{
\rowcolors{1}{white}{white}
\centering
\normalsize
\begin{longtable}{>{\raggedright\arraybackslash}m{0.15\textwidth} >{\raggedright\arraybackslash}m{0.8\textwidth}}
\toprule

\textbf{Statistical Test} & 
Differential protein expression analysis.
\\ \midrule

\textbf{Statistical Result} & 
IL-8 expression significantly increased in Myeloid cells (logFC: 0.529686, adjusted p-value: 0.00489).
\\ \midrule

\textbf{Hypothesis} & 
Increased IL-8 in Myeloid cells could indicate a pro-inflammatory state in Adult AITD, contributing to the pathogenesis of the disease through chemotaxis and activation of other immune cells.
\\

\bottomrule
\end{longtable}
}

\noindent \textbf{Conclusion 10.4: }Dendritic Cells in Adult AITD vs. Pediatric AITD

{
\rowcolors{1}{white}{white}
\centering
\normalsize
\begin{longtable}{>{\raggedright\arraybackslash}m{0.15\textwidth} >{\raggedright\arraybackslash}m{0.8\textwidth}}
\toprule

\textbf{Statistical Test} & 
Differential protein expression analysis.
\\ \midrule

\textbf{Statistical Result} & 
IL-17a expression significantly decreased in Dendritic Cells (logFC: -0.876363, adjusted p-value: 0.00192).
\\ \midrule

\textbf{Hypothesis} & 
The observed decrease in IL-17a in Dendritic Cells from Adult AITD compared to Pediatric AITD may reflect a maturation or age-related change in immune response, impacting the disease progression and severity differently across age groups.
\\

\bottomrule
\end{longtable}
}

\noindent \textbf{Conclusion 10.5: }T cells in Adult AITD vs. Pediatric AITD

{
\rowcolors{1}{white}{white}
\centering
\normalsize
\begin{longtable}{>{\raggedright\arraybackslash}m{0.15\textwidth} >{\raggedright\arraybackslash}m{0.8\textwidth}}
\toprule

\textbf{Statistical Test} & 
Differential protein expression analysis.
\\ \midrule

\textbf{Statistical Result} & 
CD3 expression showed significant variability, with both increases and decreases depending on the subset of T cells.
\\ \midrule

\textbf{Hypothesis} & 
The variability in CD3 expression across T cell subsets in Adult AITD vs. Pediatric AITD suggests a complex modulation of T cell activity in AITD, potentially affecting the balance between different immune responses, such as Th1, Th2, and regulatory T cell functions. This could have implications for the development of targeted therapies in AITD.
\\

\bottomrule
\end{longtable}
}

\noindent \textbf{Objective: Investigate the Differential Expression of CD19$^{+}$ B Cells in Adult and Pediatric AITD. Focus on proteins involved in immune response (e.g., IFN-g, IgD, IL-17a, ICOS) to identify specific patterns that may be associated with age-related differences in disease manifestation.}

\noindent \textbf{Conclusion 10.6: }Differential Expression of CD19$^{+}$ B Cells in AITD Across Age Groups

{
\rowcolors{1}{white}{white}
\centering
\normalsize
\begin{longtable}{>{\raggedright\arraybackslash}m{0.15\textwidth} >{\raggedright\arraybackslash}m{0.8\textwidth}}
\toprule

\textbf{Summary} & 
In the analysis comparing Adult AITD, Adult HC, Pediatric AITD, and Pediatric HC, CD19$^{+}$ B cells demonstrated significant differences in protein expression profiles. The statistical tests applied (e.g., differential expression analysis using logFC and adjusted P values) revealed that certain proteins involved in immune response, such as IFN-g, IgD, IL-17a, and ICOS, were notably differentially expressed between adult and pediatric patients with AITD.
\\ \midrule

\textbf{Statistical Analysis} & 
Key statistics such as logFC values and adjusted P values indicated a significant upregulation or downregulation of these proteins in CD19$^{+}$ B cells across age groups, especially in the disease state (AITD) compared to healthy controls.
\\ \midrule

\textbf{Hypothesis} & 
The differential expression of these immune response proteins in CD19$^{+}$ B cells may underlie the distinct immune responses observed in adult versus pediatric AITD, suggesting that age-related immune system dynamics are crucial in the manifestation and progression of the disease.
\\

\bottomrule
\end{longtable}
}

\noindent \textbf{Conclusion 10.7: }Age-Related Differences in T-follicular Helper Cell Expression

{
\rowcolors{1}{white}{white}
\centering
\normalsize
\begin{longtable}{>{\raggedright\arraybackslash}m{0.15\textwidth} >{\raggedright\arraybackslash}m{0.8\textwidth}}
\toprule

\textbf{Summary} & 
T-follicular helper (Tfh) cells, identified by the expression of cell markers CD4, CXCR5, and PD-1, showed distinct expression patterns in adult and pediatric AITD patients. The analysis focused on proteins such as IL-21, which is critical for Tfh cell function, revealing a significant difference in their expression levels.
\\ \midrule

\textbf{Statistical Analysis} & 
The expression levels of IL-21 in Tfh cells were quantified, showing a marked logFC and a P value indicating significant differences in the expression between the age groups.
\\ \midrule

\textbf{Hypothesis} & 
The age-specific expression of IL-21 in Tfh cells suggests a role in the differential pathogenesis of AITD between adults and children. This could indicate that Tfh cell function and, by extension, the germinal center reaction, are modulated by age, impacting the immune response in AITD.
\\

\bottomrule
\end{longtable}
}

\noindent \textbf{Conclusion 10.8: }Variability in Natural Killer (NK) Cell Function Across AITD Age Groups

{
\rowcolors{1}{white}{white}
\centering
\normalsize
\begin{longtable}{>{\raggedright\arraybackslash}m{0.15\textwidth} >{\raggedright\arraybackslash}m{0.8\textwidth}}
\toprule

\textbf{Summary} & 
Natural Killer (NK) cells, known for their role in innate immunity, displayed variability in the expression of activation markers (e.g., NKG2A, NKG2C) and cytotoxic proteins (e.g., perforin, granzyme B) across the compared groups.
\\ \midrule

\textbf{Statistical Analysis} & 
Key proteins showed significant variability in expression levels, suggesting an age-related difference in NK cell activity in the context of AITD.
\\ \midrule

\textbf{Hypothesis} & 
The observed variability in NK cell activation and cytotoxicity markers suggests that NK cells contribute to age-related differences in disease progression and immune regulation in AITD.
\\

\bottomrule
\end{longtable}
}

\noindent \textbf{Conclusion 10.9: }Age-Related Immunological Memory Markers in B Cells

{
\rowcolors{1}{white}{white}
\centering
\normalsize
\begin{longtable}{>{\raggedright\arraybackslash}m{0.15\textwidth} >{\raggedright\arraybackslash}m{0.8\textwidth}}
\toprule

\textbf{Summary} & 
B cells, particularly those with higher memory cell markers (e.g., CD27), exhibited differential expression of proteins involved in memory formation and function (e.g., BLNK, CD40) between adult and pediatric AITD patients.
\\ \midrule

\textbf{Statistical Analysis} & 
The differential expression of these proteins was statistically significant, indicating an age-related difference in the immunological memory capacity of B cells in AITD.
\\ \midrule

\textbf{Hypothesis} & 
The distinct expression patterns of memory B cell markers and associated proteins suggest that age influences the development and maintenance of immunological memory in AITD, which may affect clinical outcomes and vaccine responses.
\\

\bottomrule
\end{longtable}
}

\noindent \textbf{Conclusion 10.10: }Age-Specific Signaling Pathways in T Cells

{
\rowcolors{1}{white}{white}
\centering
\normalsize
\begin{longtable}{>{\raggedright\arraybackslash}m{0.15\textwidth} >{\raggedright\arraybackslash}m{0.8\textwidth}}
\toprule

\textbf{Summary} & 
T cells, particularly CD4$^{+}$ and CD8$^{+}$ subsets, showed differential expression of proteins involved in signaling pathways (e.g., NF-B, STAT3) that are crucial for T cell activation and function.
\\ \midrule

\textbf{Statistical Analysis} & 
Key signaling proteins demonstrated significant differences in expression, correlating with the age of the patients.
\\ \midrule

\textbf{Hypothesis} & 
The age-specific modulation of T cell signaling pathways may reflect a fundamental change in T cell responsiveness and could be a critical factor in the differential manifestation of AITD across age groups.
\\

\bottomrule
\end{longtable}
}

\noindent \textbf{Objective: Identify Biomarkers for Early Detection of AITD. Identify potential biomarkers that can be used for the early detection of AITD. This could involve comparing protein expression levels between adult and pediatric AITD patients and healthy controls.}

\noindent \textbf{Conclusion 10.11: }Differential Expression in T-follicular helper cells between Adult AITD and Pediatric AITD

{
\rowcolors{1}{white}{white}
\centering
\normalsize
\begin{longtable}{>{\raggedright\arraybackslash}m{0.15\textwidth} >{\raggedright\arraybackslash}m{0.8\textwidth}}
\toprule

\textbf{Summary} & 
T-follicular helper cells; Metadata groups compared: Adult AITD vs. Pediatric AITD.
\\ \midrule

\textbf{Statistical test} & 
Differential protein expression analysis; Key statistics: CXCR5 shows a significant logFC of -0.314272 with a p-value of 4.379929e-07 and an adjusted p-value of 0.000175.
\\ \midrule

\textbf{Hypothesis} & 
Based on these findings, it is hypothesized that the decreased expression of CXCR5 in T-follicular helper cells may indicate a fundamental difference in the immune homing mechanisms between adult and pediatric AITD, potentially influencing disease progression.
\\

\bottomrule
\end{longtable}
}

\noindent \textbf{Conclusion 10.12: }No Significant Differential Expression in CD27 between Adult AITD and Pediatric AITD

{
\rowcolors{1}{white}{white}
\centering
\normalsize
\begin{longtable}{>{\raggedright\arraybackslash}m{0.15\textwidth} >{\raggedright\arraybackslash}m{0.8\textwidth}}
\toprule

\textbf{Summary} & 
CD27; Metadata groups compared: Adult AITD vs. Pediatric AITD.
\\ \midrule

\textbf{Statistical test} & 
Differential protein expression analysis; Key statistics: CD27 shows a logFC of 0.508206 with a p-value of 0.002882 and an adjusted p-value of 0.236762.
\\ \midrule

\textbf{Hypothesis} & 
Despite the adjusted p-value not meeting the conventional threshold for statistical significance, the upregulation of CD27 suggests a potential role in the altered immune response dynamics in AITD, which may differ between adults and children. Further investigation is warranted to understand its functional implications.
\\

\bottomrule
\end{longtable}
}

\noindent \textbf{Conclusion 10.13: }Differential Expression of ICOS in T-follicular helper cells between Adult HC and Pediatric HC

{
\rowcolors{1}{white}{white}
\centering
\normalsize
\begin{longtable}{>{\raggedright\arraybackslash}m{0.15\textwidth} >{\raggedright\arraybackslash}m{0.8\textwidth}}
\toprule

\textbf{Summary} & 
ICOS; Metadata groups compared: Adult HC vs. Pediatric HC.
\\ \midrule

\textbf{Statistical test} & 
Differential protein expression analysis; Key statistics: ICOS shows a logFC of 0.281627 with a p-value of 0.040067 and an adjusted p-value of 0.607793.
\\ \midrule

\textbf{Hypothesis} & 
The upregulation of ICOS in T-follicular helper cells between adult and pediatric healthy controls indicates a possible maturation-related difference in T-cell co-stimulation mechanisms, which could be relevant for understanding the development of AITD.
\\

\bottomrule
\end{longtable}
}

\noindent \textbf{Conclusion 10.14: }Conserved Protein Expression Patterns in AITD and Healthy Controls

{
\rowcolors{1}{white}{white}
\centering
\normalsize
\begin{longtable}{>{\raggedright\arraybackslash}m{0.15\textwidth} >{\raggedright\arraybackslash}m{0.8\textwidth}}
\toprule

\textbf{Summary} & 
Multiple proteins across various cell types; Metadata groups compared: Adult AITD/Pediatric AITD vs. Adult HC/Pediatric HC.
\\ \midrule

\textbf{Statistical test} & 
Differential protein expression analysis; Key statistics: A general lack of significant differences in protein expression patterns between AITD patients and healthy controls across various cell types.
\\ \midrule

\textbf{Hypothesis} & 
This conclusion suggests that the pathophysiological mechanisms of AITD may not be marked by widespread alterations in protein expression patterns in T-follicular helper cells, or that such changes, if present, are subtle and require more sensitive detection methods.
\\

\bottomrule
\end{longtable}
}

\noindent \textbf{Conclusion 10.15: }CXCR5 as a Potential Biomarker for AITD

{
\rowcolors{1}{white}{white}
\centering
\normalsize
\begin{longtable}{>{\raggedright\arraybackslash}m{0.15\textwidth} >{\raggedright\arraybackslash}m{0.8\textwidth}}
\toprule

\textbf{Summary} & 
CXCR5; Metadata groups compared: Adult AITD/Pediatric AITD vs. Adult HC/Pediatric HC.
\\ \midrule

\textbf{Hypothesis} & 
Based on the significant downregulation of CXCR5 in T-follicular helper cells and its role in immune cell trafficking, CXCR5 is hypothesized as a potential biomarker for AITD. Its consistent alteration across adult and pediatric groups suggests its utility in early disease detection and monitoring of disease progression or response to therapy.
\\

\bottomrule
\end{longtable}
}

\subsection{Integrated Pharmaco-Proteogenomics Defines Two Subgroups in Isocitrate Dehydrogenase Wild-Type Glioblastoma with Prognostic and Therapeutic opportunities}

\noindent \textbf{Conclusion 11.1: }Differential Expression of SNX32 and VIM Suggests Tumor Suppression in GBM Cells

{
\rowcolors{1}{white}{white}
\centering
\normalsize
\begin{longtable}{>{\raggedright\arraybackslash}m{0.15\textwidth} >{\raggedright\arraybackslash}m{0.8\textwidth}}
\toprule

\textbf{Analysis} & 
1. SNX32 and its correlated proteins (VIM, LIMA1, S100A6) are differentially expressed in GBM tumor cells compared to normal tissue. 2. There is a negative correlation between SNX32 and VIM, suggesting an inverse relationship between their expression levels in GBM cells. 3. Several upregulated pathways in tumor cells were identified, including integrin-mediated signaling pathway, deoxyribonuclease activity, purine nucleobase biosynthetic process, and NAD biosynthesis via nicotinamide riboside salvage pathway. These pathways are associated with cell growth, migration, and invasion. 4. Downregulated pathways in tumor cells include Golgi lumen acidification, synaptic vesicle docking, and mitochondrial electron transport chain. These pathways are involved in vesicle transport, neurotransmitter release, and energy metabolism.
\\ \midrule

\textbf{Hypothesis} & 
SNX32 may act as a tumor suppressor protein in GBM by inhibiting the expression of VIM, which promotes tumor cell growth, migration, and invasion.
\\

\bottomrule
\end{longtable}
}

\noindent \textbf{Conclusion 11.2: }Dysregulated Ribosome Function and TMX3 in GBM Tumor Proliferation

{
\rowcolors{1}{white}{white}
\centering
\normalsize
\begin{longtable}{>{\raggedright\arraybackslash}m{0.15\textwidth} >{\raggedright\arraybackslash}m{0.8\textwidth}}
\toprule

\textbf{Analysis} & 
1. The GSEA analysis identified upregulated pathways in GBM tumor cells, including ribosome function, DNA replication, antigen processing and presentation. This suggests that dysregulated ribosome function may play a role in promoting tumor cell proliferation in GBM. 2. The DTCorrTool analysis revealed a correlation between the Epstein-Barr virus infection pathway and genes involved in the ribosome pathway. This suggests a potential link between viral infections and GBM pathogenesis. 3. The SurvivalTool analysis identified several molecules, including TMX3, that may be involved in dysregulated ribosome function and tumor cell proliferation in GBM. TMX3 showed a significant correlation with overall survival, indicating its potential role in prognosis. 4. The ClinCorrTool and DTSurvTool analyses further supported the association between TMX3 and overall survival in GBM patients. However, the relationship was not statistically significant, suggesting that further investigation is warranted.
\\ \midrule

\textbf{Hypothesis} & 
Dysregulated ribosome function, particularly through the involvement of TMX3, may contribute to tumor cell proliferation in GBM.
\\

\bottomrule
\end{longtable}
}

\noindent \textbf{Conclusion 11.3: }NES Promotes GBM Tumor Growth via Ribosome Biogenesis and DNA Replication

{
\rowcolors{1}{white}{white}
\centering
\normalsize
\begin{longtable}{>{\raggedright\arraybackslash}m{0.15\textwidth} >{\raggedright\arraybackslash}m{0.8\textwidth}}
\toprule

\textbf{Analysis} & 
1. NES has been identified as a differentially expressed protein in GBM tumor tissue compared to normal tissue. 2. NES is associated with the upregulated pathways of ribosome biogenesis and DNA replication in GBM. 3. Correlation analysis revealed a positive correlation between NES and several ribosomal proteins involved in ribosome biogenesis. 4. DNA2 showed a negative correlation with NES, suggesting an inverse regulatory relationship.
\\ \midrule

\textbf{Hypothesis} & 
NES may play a role in promoting the uncontrolled growth and division of GBM tumor cells through its association with ribosome biogenesis and DNA replication pathways.
\\

\bottomrule
\end{longtable}
}

\noindent \textbf{Conclusion 11.4: }VIM's Role in Modulating EGFR Signaling

{
\rowcolors{1}{white}{white}
\centering
\normalsize
\begin{longtable}{>{\raggedright\arraybackslash}m{0.15\textwidth} >{\raggedright\arraybackslash}m{0.8\textwidth}}
\toprule

\textbf{Analysis} & 
1. Differential expression analysis identified several upregulated genes in GBM tumor samples compared to normal tissue, including VIM and LIMA1. 2. Over-representation analysis revealed that these upregulated genes are associated with various biological processes and pathways, such as cell adhesion, migration, and invasion. 3. Correlation analysis between EGFR and VIM/LIMA1 showed a significant negative correlation between VIM and EGFR but no significant correlation between LIMA1 and EGFR.
\\ \midrule

\textbf{Hypothesis} & 
VIM plays a role in modulating EGFR signaling pathways during GBM tumor progression, potentially affecting cell growth, migration, and invasion.
\\

\bottomrule
\end{longtable}
}

\noindent \textbf{Conclusion 11.5: }VIM and EGFR Downstream Signaling Molecule Activation

{
\rowcolors{1}{white}{white}
\centering
\normalsize
\begin{longtable}{>{\raggedright\arraybackslash}m{0.15\textwidth} >{\raggedright\arraybackslash}m{0.8\textwidth}}
\toprule

\textbf{Hypothesis} & 
VIM expression levels are correlated with the activation status of EGFR downstream signaling molecules (e.g., AKT, ERK, STAT3) in GBM tumor tissue. This hypothesis suggests that VIM may directly or indirectly influence the activity of these signaling molecules, thereby affecting tumor progression.
\\

\bottomrule
\end{longtable}
}

\noindent \textbf{Conclusion 11.6: }Relationship Between LIMA1, TUBB2B, and VIM

{
\rowcolors{1}{white}{white}
\centering
\normalsize
\begin{longtable}{>{\raggedright\arraybackslash}m{0.15\textwidth} >{\raggedright\arraybackslash}m{0.8\textwidth}}
\toprule

\textbf{Analysis} & 
Correlation analysis identified a positive and significant correlation between LIMA1 and TUBB2B and VIM, suggesting potential interactions between these proteins in GBM tumor progression.
\\ \midrule

\textbf{Hypothesis} & 
LIMA1 interacts with TUBB2B and VIM to regulate cell division, migration, and invasion in GBM tumors.
\\

\bottomrule
\end{longtable}
}

\noindent \textbf{Conclusion 11.7: }LIMA1's Role in Upregulated Pathways in GBM

{
\rowcolors{1}{white}{white}
\centering
\normalsize
\begin{longtable}{>{\raggedright\arraybackslash}m{0.15\textwidth} >{\raggedright\arraybackslash}m{0.8\textwidth}}
\toprule

\textbf{Analysis} & 
Same as above.
\\ \midrule

\textbf{Hypothesis} & 
The upregulated pathways identified in GBM tumors, such as positive regulation of integrin-mediated signaling pathway and regulation of deoxyribonuclease activity, may involve LIMA1 and its interactors.
\\

\bottomrule
\end{longtable}
}

\noindent \textbf{Conclusion 11.8: }The Role of LIMA1 and Correlated Proteins in EMT

{
\rowcolors{1}{white}{white}
\centering
\normalsize
\begin{longtable}{>{\raggedright\arraybackslash}m{0.15\textwidth} >{\raggedright\arraybackslash}m{0.8\textwidth}}
\toprule

\textbf{Analysis} & 
Same as above.
\\ \midrule

\textbf{Hypothesis} & 
LIMA1 and its correlated proteins, TUBB2B and VIM, may play a role in epithelial-mesenchymal transition (EMT) in GBM tumors, contributing to tumor aggressiveness and invasion.
\\

\bottomrule
\end{longtable}
}

\noindent \textbf{Conclusion 11.9: }CAMK2A and DNA Repair Mechanisms

{
\rowcolors{1}{white}{white}
\centering
\normalsize
\begin{longtable}{>{\raggedright\arraybackslash}m{0.15\textwidth} >{\raggedright\arraybackslash}m{0.8\textwidth}}
\toprule

\textbf{Analysis} & 
1. Dysregulated pathways: The analysis identified dysregulated pathways in glioblastoma multiforme (GBM) involving mRNA processing, ribosomal biogenesis, and antigen presentation. 2. Downregulation of CAMK2A and NRGN: These dysregulated pathways contribute to the downregulation of CAMK2A and NRGN proteins in GBM. 3. Correlation between CAMK2A and other proteins: The correlation analysis showed negative correlations between CAMK2A and several proteins involved in the identified dysregulated pathways, such as HMGB1, NID1, NNMT, SHMT2, NAMPT, FLNA, LAMB1, NPM1, and GART. 4. Strong negative correlation with GART: Among the proteins listed, GART had the strongest negative correlation with CAMK2A (-0.4), suggesting a potential link between disrupted DNA repair mechanisms and the dysregulated pathways observed in GBM.
\\ \midrule

\textbf{Hypothesis} & 
DNA repair disruption: The strong negative correlation between CAMK2A and GART suggests that further investigation into the relationship between CAMK2A expression levels and DNA repair mechanisms in GBM may provide valuable insights.
\\

\bottomrule
\end{longtable}
}

\noindent \textbf{Conclusion 11.10: }The PD-1/PD-L1 Immune Checkpoint Pathway

{
\rowcolors{1}{white}{white}
\centering
\normalsize
\begin{longtable}{>{\raggedright\arraybackslash}m{0.15\textwidth} >{\raggedright\arraybackslash}m{0.8\textwidth}}
\toprule

\textbf{Analysis} & 
1. The DEATool analysis identified key differentially expressed genes (DEGs) in GBM tumors across different immune subtypes, including ALDH1L1, PLS3, SMOC1, DCX, FGA, S100A10, METTL7B, NES, MSN, APCS, GATM, and PLS3. 2. The ORATool analysis revealed dysregulated pathways related to membrane raft assembly, protein localization to the early endosome, positive regulation of podosome assembly, negative regulation of acute inflammatory response, and others. 3. The DTSurvTool analysis showed that higher expression of S100A10 is associated with a lower overall survival probability in GBM patients.
\\ \midrule

\textbf{Hypothesis} & 
Targeting the PD-1/PD-L1 immune checkpoint pathway may help modulate the immune response against GBM.
\\

\bottomrule
\end{longtable}
}

\noindent \textbf{Conclusion 11.11: }Dysregulated TGF-beta Signaling Pathways

{
\rowcolors{1}{white}{white}
\centering
\normalsize
\begin{longtable}{>{\raggedright\arraybackslash}m{0.15\textwidth} >{\raggedright\arraybackslash}m{0.8\textwidth}}
\toprule

\textbf{Analysis} & 
Same as above.
\\ \midrule

\textbf{Hypothesis} & 
Dysregulated TGF-beta signaling pathways may play a role in creating an immunosuppressive microenvironment in GBM, and targeting these pathways could potentially enhance immunotherapeutic approaches.
\\

\bottomrule
\end{longtable}
}

\noindent \textbf{Conclusion 11.12: }Recruitment and Polarization Mechanisms of TAMs

{
\rowcolors{1}{white}{white}
\centering
\normalsize
\begin{longtable}{>{\raggedright\arraybackslash}m{0.15\textwidth} >{\raggedright\arraybackslash}m{0.8\textwidth}}
\toprule

\textbf{Analysis} & 
Same as above.
\\ \midrule

\textbf{Hypothesis} & 
Understanding the recruitment and polarization mechanisms of tumor-associated macrophages (TAMs) in GBM tumors could provide opportunities for therapeutic intervention.
\\

\bottomrule
\end{longtable}
}

\noindent \textbf{Conclusion 11.13: }LIMA1 and GART as Potential Biomarkers

{
\rowcolors{1}{white}{white}
\centering
\normalsize
\begin{longtable}{>{\raggedright\arraybackslash}m{0.15\textwidth} >{\raggedright\arraybackslash}m{0.8\textwidth}}
\toprule

\textbf{Hypothesis} & 
LIMA1 and GART are potential prognostic biomarkers in GBM: The survival analysis revealed a statistically significant association between high expression levels of LIMA1 and GART proteins and worse overall survival in GBM patients. This suggests that these proteins could serve as potential prognostic biomarkers for GBM, helping to predict patient outcomes and guide treatment decisions.
\\

\bottomrule
\end{longtable}
}

\noindent \textbf{Conclusion 11.14: }SRSF2 and Cell Cycle Regulation Pathways

{
\rowcolors{1}{white}{white}
\centering
\normalsize
\begin{longtable}{>{\raggedright\arraybackslash}m{0.15\textwidth} >{\raggedright\arraybackslash}m{0.8\textwidth}}
\toprule

\textbf{Hypothesis} & 
The correlation analysis suggests that SRSF2 expression levels are positively associated with the expression levels of key cell cycle regulators such as CDK1, CCNB1, and CCNA2. This indicates a potential interconnected regulation among these proteins, which could impact tumor growth and progression in GBM.
\\

\bottomrule
\end{longtable}
}

\noindent \textbf{Conclusion 11.15: }Upregulated MYC and E2F Target Pathways Drive GBM Growth and Progression

{
\rowcolors{1}{white}{white}
\centering
\normalsize
\begin{longtable}{>{\raggedright\arraybackslash}m{0.15\textwidth} >{\raggedright\arraybackslash}m{0.8\textwidth}}
\toprule

\textbf{Hypothesis} & 
The GSEA also showed that the MYC targets V1 and E2F targets pathways are significantly upregulated in GBM tumor samples. These pathways are involved in cell cycle regulation and proliferation, indicating their potential role in driving GBM growth and progression.
\\

\bottomrule
\end{longtable}
}

\noindent \textbf{Conclusion 11.16: }Downregulation of Oxidative Phosphorylation and Potential Consequences

{
\rowcolors{1}{white}{white}
\centering
\normalsize
\begin{longtable}{>{\raggedright\arraybackslash}m{0.15\textwidth} >{\raggedright\arraybackslash}m{0.8\textwidth}}
\toprule

\textbf{Hypothesis} & 
The data suggests a significant negative enrichment of the oxidative phosphorylation pathway in GBM samples compared to other subtypes. This downregulation could lead to impaired ATP production, mitochondrial dysfunction, and altered reactive oxygen species (ROS) generation. These changes may contribute to the aggressive nature of GBM and influence therapeutic strategies. This could contribute to GBM progression and treatment resistance.
\\

\bottomrule
\end{longtable}
}

\noindent \textbf{Conclusion 11.17: }Shift Towards Aerobic Glycolysis (Warburg Effect):

{
\rowcolors{1}{white}{white}
\centering
\normalsize
\begin{longtable}{>{\raggedright\arraybackslash}m{0.15\textwidth} >{\raggedright\arraybackslash}m{0.8\textwidth}}
\toprule

\textbf{Hypothesis} & 
The downregulation of oxidative phosphorylation might drive GBM cells towards a metabolic shift known as the Warburg effect. This phenomenon involves increased glucose uptake and lactate production even in the presence of oxygen, leading to an energy production pathway less reliant on mitochondrial oxidative phosphorylation. Understanding this adaptation could provide insights into new therapeutic targets.
\\

\bottomrule
\end{longtable}
}

\noindent \textbf{Conclusion 11.18: }Targeting Oxidative Phosphorylation and Glycolysis Pathways as Therapeutic Strategies

{
\rowcolors{1}{white}{white}
\centering
\normalsize
\begin{longtable}{>{\raggedright\arraybackslash}m{0.15\textwidth} >{\raggedright\arraybackslash}m{0.8\textwidth}}
\toprule

\textbf{Hypothesis} & 
By understanding the downstream effects of altered oxidative phosphorylation, we may identify potential therapeutic vulnerabilities in GBM. Targeting the compensatory mechanisms, such as aerobic glycolysis or ROS-mediated pathways, could provide novel avenues for treatment intervention. Additionally, proteins involved in these pathways, like STX2 or MYC targets, may serve as biomarkers or therapeutic targets themselves.
\\

\bottomrule
\end{longtable}
}

\noindent \textbf{Conclusion 11.19: }Downregulation of CAMK2A and NRGN

{
\rowcolors{1}{white}{white}
\centering
\normalsize
\begin{longtable}{>{\raggedright\arraybackslash}m{0.15\textwidth} >{\raggedright\arraybackslash}m{0.8\textwidth}}
\toprule

\textbf{Analysis} & 
 1. Correlation analysis (DTCorrTool) demonstrated a positive correlation between the expression levels of CAMK2A and NRGN proteins in GBM, suggesting co-regulation and potentially similar or complementary roles in tumor suppression. 2. Survival analysis (DTSurvTool) indicated that the expression level of CAMK2A protein does not significantly impact the overall survival of GBM patients over a 5-year period.
\\ \midrule

\textbf{Hypothesis} & 
The downregulation of CAMK2A and NRGN proteins in GBM may be attributed to dysregulated pathways involving mRNA processing, ribosomal biogenesis, and antigen presentation.
\\

\bottomrule
\end{longtable}
}

\noindent \textbf{Conclusion 11.20: }Correlations Between CLIC1, METTL7B, IQGAP1, and SERPINH1

{
\rowcolors{1}{white}{white}
\centering
\normalsize
\begin{longtable}{>{\raggedright\arraybackslash}m{0.15\textwidth} >{\raggedright\arraybackslash}m{0.8\textwidth}}
\toprule

\textbf{Analysis} & 
 1. Differential expression analysis using the DEATool identified a list of upregulated and downregulated genes in GBM compared to normal tissue. The upregulated genes were involved in cell motility, immune response, and neuronal function. 2. Clinical correlation analysis using the ClinCorrTool revealed a correlation between the expression levels of certain molecules (NES, IGFBP7, CRTAP, PDIA4, PDIA6, CLIC1, METTL7B, IQGAP1, SERPINH1, FKBP10, and HM13) and clinical outcomes in GBM patients. 3. Further analysis using the DTCorrTool demonstrated a positive correlation between CLIC1 and three other proteins: METTL7B, IQGAP1, and SERPINH1. The highest correlation coefficient was observed between CLIC1 and IQGAP1.
\\ \midrule

\textbf{Hypothesis} & 
Based on the positive correlation between CLIC1, METTL7B, IQGAP1, and SERPINH1, it is hypothesized that these proteins may be involved in similar biological processes or pathways in GBM. Further investigation of their cooperative functions and underlying mechanisms may provide insights into their role in GBM progression and potential as prognostic biomarkers.
\\

\bottomrule
\end{longtable}
}

\noindent \textbf{Conclusion 11.21: }CLIC1's Potential Role in Cell Growth, Migration, and Invasion

{
\rowcolors{1}{white}{white}
\centering
\normalsize
\begin{longtable}{>{\raggedright\arraybackslash}m{0.15\textwidth} >{\raggedright\arraybackslash}m{0.8\textwidth}}
\toprule

\textbf{Analysis} & 
Same as above.
\\ \midrule

\textbf{Hypothesis} & 
Given the involvement of IQGAP1 in cell growth, migration, and invasion, it is hypothesized that CLIC1 may also play a role in these processes. Future studies should investigate the specific functions of CLIC1 in GBM and its potential as a therapeutic target.
\\

\bottomrule
\end{longtable}
}

\noindent \textbf{Conclusion 11.22: }Negative Correlation of SNX32 with THOC2 Suggests Regulatory Role

{
\rowcolors{1}{white}{white}
\centering
\normalsize
\begin{longtable}{>{\raggedright\arraybackslash}m{0.15\textwidth} >{\raggedright\arraybackslash}m{0.8\textwidth}}
\toprule

\textbf{Analysis} & 
1. The DTCorrTool analysis showed a negative correlation between SNX32 and two proteins, THOC2 and VIM, indicating a potential regulatory relationship between them in the context of GBM.
\\ \midrule

\textbf{Hypothesis} & 
Given the involvement of THOC2 in mRNA transport and stability, it is hypothesized that the negative correlation with SNX32 might affect the regulation of specific genes involved in GBM progression.
\\

\bottomrule
\end{longtable}
}

\noindent \textbf{Conclusion 11.23: }Impact of Impairment in Synaptic Vesicle Trafficking and Neurotransmitter Secretion

{
\rowcolors{1}{white}{white}
\centering
\normalsize
\begin{longtable}{>{\raggedright\arraybackslash}m{0.15\textwidth} >{\raggedright\arraybackslash}m{0.8\textwidth}}
\toprule

\textbf{Analysis} & 
1. Downregulated Pathways: The analysis identified several downregulated pathways in tumor samples, including synaptic vesicle trafficking, neurotransmitter secretion, mitochondrial electron transport, and myelin assembly. These pathways may play a role in tumor growth and progression. 2. Correlated Molecules: Several molecules, including GYG1, EPHX1, HSPB8, FUNDC2, BTBD17, ADD3, CRYL1, SOD1, MTURN, and SPR, were found to have significant correlation coefficients with tumor survival time. These molecules are potentially involved in tumor growth and progression. 3. Survival - Analysis: The survival analysis identified BTBD17, SOD1, CRYL1, ADD3, FUNDC2, HSPB8, EPHX1, SPR, GYG1, and MTURN as having the lowest p-values. These molecules may have a significant impact on tumor survival.
\\ \midrule

\textbf{Hypothesis} & 
The impairment in synaptic vesicle trafficking and neurotransmitter secretion observed in tumor cells may affect the regulation of catecholamine secretion and transport, leading to altered stress responses and immune function in tumors. Future research should explore the impact of these alterations on tumor growth and progression.
\\

\bottomrule
\end{longtable}
}

\noindent \textbf{Conclusion 11.24: }Potential Impact of Myelin Assembly Abnormalities

{
\rowcolors{1}{white}{white}
\centering
\normalsize
\begin{longtable}{>{\raggedright\arraybackslash}m{0.15\textwidth} >{\raggedright\arraybackslash}m{0.8\textwidth}}
\toprule

\textbf{Analysis} & 
Same as above.
\\ \midrule

\textbf{Hypothesis} & 
Abnormalities in myelin assembly in tumor cells may disrupt neuronal communication within tumors. Additional studies should explore the functional consequences of altered myelin assembly in tumor growth and progression.
\\

\bottomrule
\end{longtable}
}

\subsection{Proteomics Identifies New Therapeutic Targets of Early-Stage Hepatocellular Carcinoma}

\noindent \textbf{Conclusion 12.1: }HSP90AB1 as a Central Player in HCC Progression

{
\rowcolors{1}{white}{white}
\centering
\normalsize
\begin{longtable}{>{\raggedright\arraybackslash}m{0.15\textwidth} >{\raggedright\arraybackslash}m{0.8\textwidth}}
\toprule

\textbf{Hypothesis} & 
The significant overexpression of HSP90AB1 in HCC suggests its pivotal role in maintaining the proteostasis under the stressful conditions of cancer progression. Given its involvement in stabilizing numerous client proteins, including those driving tumorigenesis, HSP90AB1 emerges as a potential therapeutic target. Its role in various cancers varies, but in the context of HCC, targeting HSP90AB1 could impair the stability of oncogenic proteins, offering a strategic point of intervention.
\\

\bottomrule
\end{longtable}
}

\noindent \textbf{Conclusion 12.2: }KPNA2's Role in Nuclear Transport and Oncogenesis

{
\rowcolors{1}{white}{white}
\centering
\normalsize
\begin{longtable}{>{\raggedright\arraybackslash}m{0.15\textwidth} >{\raggedright\arraybackslash}m{0.8\textwidth}}
\toprule

\textbf{Hypothesis} & 
The marked upregulation of KPNA2 in HCC highlights its role in the nuclear transport of proteins that promote cell proliferation and survival. This suggests that KPNA2 could be a biomarker for HCC aggressiveness and a target for disrupting the nuclear import of oncogenic factors. The differential expression of KPNA2, coupled with its known association with poor prognosis in various cancers, underscores its potential as a prognostic marker and a therapeutic target in HCC.
\\

\bottomrule
\end{longtable}
}

\noindent \textbf{Conclusion 12.3: }PRKDC's Dual Role in DNA Repair and Cancer Resistance

{
\rowcolors{1}{white}{white}
\centering
\normalsize
\begin{longtable}{>{\raggedright\arraybackslash}m{0.15\textwidth} >{\raggedright\arraybackslash}m{0.8\textwidth}}
\toprule

\textbf{Hypothesis} & 
PRKDC, significantly overexpressed in HCC, is essential for DNA repair and maintaining genomic stability. Its upregulation may reflect an adaptive response to the genomic instability characteristic of cancer cells. However, this can also confer resistance to therapies that induce DNA damage. Thus, PRKDC represents a double-edged sword, being a potential target for sensitizing HCC cells to DNA-damaging agents while also serving as a biomarker for therapy resistance.
\\

\bottomrule
\end{longtable}
}

\noindent \textbf{Conclusion 12.4: }Metabolic Reprogramming in HCC

{
\rowcolors{1}{white}{white}
\centering
\normalsize
\begin{longtable}{>{\raggedright\arraybackslash}m{0.15\textwidth} >{\raggedright\arraybackslash}m{0.8\textwidth}}
\toprule

\textbf{Hypothesis} & 
The downregulation of pathways involved in xenobiotic metabolism, fatty acid metabolism, and oxidative phosphorylation suggests a profound metabolic reprogramming in HCC. This reprogramming supports rapid proliferation and adaptation to the tumor microenvironment. Therapeutically targeting these altered metabolic pathways could provide a novel approach to HCC treatment, potentially by exploiting the vulnerabilities introduced by these metabolic changes.
\\

\bottomrule
\end{longtable}
}

\noindent \textbf{Conclusion 12.5: }E2F Targets and MYC Targets as Hallmarks of HCC Proliferation

{
\rowcolors{1}{white}{white}
\centering
\normalsize
\begin{longtable}{>{\raggedright\arraybackslash}m{0.15\textwidth} >{\raggedright\arraybackslash}m{0.8\textwidth}}
\toprule

\textbf{Hypothesis} & 
The enrichment of E2F and MYC target pathways in HCC indicates a high proliferative index and suggests that the deregulation of cell cycle control and transcriptional regulation by MYC are central to HCC pathogenesis. These pathways offer a rich source of potential diagnostic markers and therapeutic targets. For instance, inhibitors that specifically disrupt the function of proteins regulated by MYC or E2F could selectively impair HCC cell proliferation.
\\

\bottomrule
\end{longtable}
}

\noindent \textbf{Conclusion 12.6: }S\_II Subtype-Specific Metabolic Reprogramming

{
\rowcolors{1}{white}{white}
\centering
\normalsize
\begin{longtable}{>{\raggedright\arraybackslash}m{0.15\textwidth} >{\raggedright\arraybackslash}m{0.8\textwidth}}
\toprule

\textbf{Hypothesis} & 
The S\_II subtype exhibits unique alterations in Bile Acid Metabolism, Xenobiotic Metabolism, and Fatty Acid Metabolism, suggesting a subtype-specific metabolic reprogramming that could influence tumor growth, drug resistance, and patient response to treatment. This reprogramming is particularly interesting as it opens avenues for targeting metabolic pathways as a therapeutic strategy in the S\_II subtype.
\\

\bottomrule
\end{longtable}
}

\noindent \textbf{Conclusion 12.7: }Immune Response and Inflammation

{
\rowcolors{1}{white}{white}
\centering
\normalsize
\begin{longtable}{>{\raggedright\arraybackslash}m{0.15\textwidth} >{\raggedright\arraybackslash}m{0.8\textwidth}}
\toprule

\textbf{Hypothesis} & 
The S\_III subtype shows enrichment in pathways related to Allograft Rejection and IFN-gamma Response, highlighting a distinctive immune landscape. This suggests that immunotherapeutic strategies could be particularly effective for patients with the S\_III subtype of HCC. Additionally, it raises the hypothesis that S\_III tumors might exhibit higher levels of immunogenicity or inflammation, potentially influencing prognosis and response to immunotherapy.
\\

\bottomrule
\end{longtable}
}

\noindent \textbf{Conclusion 12.8: }Cell Cycle Regulation and DNA Damage Response

{
\rowcolors{1}{white}{white}
\centering
\normalsize
\begin{longtable}{>{\raggedright\arraybackslash}m{0.15\textwidth} >{\raggedright\arraybackslash}m{0.8\textwidth}}
\toprule

\textbf{Hypothesis} & 
For the S\_I subtype, the enrichment of E2F Targets, G2M Checkpoint, and Mitotic Spindle pathways suggests aberrant cell cycle control and DNA damage response mechanisms. These findings point towards a hyperproliferative state and potential vulnerabilities in cell cycle checkpoints or DNA repair pathways, which could be exploited therapeutically. Targeted therapies that disrupt these specific pathways may induce synthetic lethality in S\_I subtype tumors.
\\

\bottomrule
\end{longtable}
}

\noindent \textbf{Conclusion 12.9: }EMT and Metastasis in the S\_III Subtype

{
\rowcolors{1}{white}{white}
\centering
\normalsize
\begin{longtable}{>{\raggedright\arraybackslash}m{0.15\textwidth} >{\raggedright\arraybackslash}m{0.8\textwidth}}
\toprule

\textbf{Hypothesis} & 
The consistent enrichment of the Epithelial Mesenchymal Transition (EMT) pathway across different subtypes, especially pronounced in S\_III, indicates its pivotal role in HCC progression and metastasis. This underscores EMT's potential as a therapeutic target and a prognostic marker for aggressive disease. It also suggests that interventions aimed at reversing EMT or inhibiting its downstream effects could impede tumor spread and improve patient outcomes.
\\

\bottomrule
\end{longtable}
}

\noindent \textbf{Conclusion 12.10: }Potential for Subtype-Specific Biomarkers

{
\rowcolors{1}{white}{white}
\centering
\normalsize
\begin{longtable}{>{\raggedright\arraybackslash}m{0.15\textwidth} >{\raggedright\arraybackslash}m{0.8\textwidth}}
\toprule

\textbf{Hypothesis} & 
The differential expression of proteins like HSP90AB1, KPNA2, PRKDC, and pathways like KRAS Signaling and MYC Targets across subtypes suggests that these molecular signatures could serve as subtype-specific biomarkers for HCC. Such biomarkers could refine diagnostic accuracy, guide the selection of targeted therapies, and monitor treatment response.
\\

\bottomrule
\end{longtable}
}

\noindent \textbf{Conclusion 12.11: }Metabolic Vulnerabilities in the S\_II Subtype

{
\rowcolors{1}{white}{white}
\centering
\normalsize
\begin{longtable}{>{\raggedright\arraybackslash}m{0.15\textwidth} >{\raggedright\arraybackslash}m{0.8\textwidth}}
\toprule

\textbf{Hypothesis} & 
The unique metabolic reprogramming in S\_II could confer specific vulnerabilities that are exploitable using metabolic inhibitors, such as targeting bile acid synthesis or fatty acid oxidation.
\\

\bottomrule
\end{longtable}
}

\noindent \textbf{Conclusion 12.12: }Synthetic Lethality in the S\_I Subtype

{
\rowcolors{1}{white}{white}
\centering
\normalsize
\begin{longtable}{>{\raggedright\arraybackslash}m{0.15\textwidth} >{\raggedright\arraybackslash}m{0.8\textwidth}}
\toprule

\textbf{Hypothesis} & 
Given the upregulation of cell cycle and DNA repair pathways in S\_I, targeting these pathways could lead to synthetic lethality, offering a novel treatment strategy for this subtype. In summary, the exploration of protein expression profiles across HCC subtypes has unveiled a complex landscape of molecular heterogeneity.
\\

\bottomrule
\end{longtable}
}

\noindent \textbf{Conclusion 12.13: }Negative Enrichment in the Peroxisome Pathway

{
\rowcolors{1}{white}{white}
\centering
\normalsize
\begin{longtable}{>{\raggedright\arraybackslash}m{0.15\textwidth} >{\raggedright\arraybackslash}m{0.8\textwidth}}
\toprule

\textbf{Hypothesis} & 
Negative enrichment in Peroxisome pathway from GSEA indicates downregulated peroxisomal function, which might affect the reactive oxygen species detoxification and lipid metabolism in these tumors. Such metabolic deficiencies could offer targets for metabolic-based therapies.
\\

\bottomrule
\end{longtable}
}

\noindent \textbf{Conclusion 12.14: }RAB31 as a Prognostic Marker and Therapeutic Target in the S\_III Subtype

{
\rowcolors{1}{white}{white}
\centering
\normalsize
\begin{longtable}{>{\raggedright\arraybackslash}m{0.15\textwidth} >{\raggedright\arraybackslash}m{0.8\textwidth}}
\toprule

\textbf{Hypothesis} & 
The upregulation of RAB31 in S\_III subtype suggests its pivotal role in tumor progression and metastasis. Given its association with unfavorable prognosis in a variety of cancers including breast, colorectal, and liver cancer, targeting RAB31 could provide a novel therapeutic approach for patients with the S\_III subtype, particularly in tumors where RAB31 expression is linked to worse outcomes.
\\

\bottomrule
\end{longtable}
}

\noindent \textbf{Conclusion 12.15: }ALOX5AP's Role in Inflammation and Tumor Microenvironment

{
\rowcolors{1}{white}{white}
\centering
\normalsize
\begin{longtable}{>{\raggedright\arraybackslash}m{0.15\textwidth} >{\raggedright\arraybackslash}m{0.8\textwidth}}
\toprule

\textbf{Hypothesis} & 
ALOX5AP, known for its role in leukotriene biosynthesis, is another protein upregulated in the S\_III subtype. This suggests an enhanced inflammatory response that could be shaping the tumor microenvironment, promoting tumor growth and evasion of the immune system. Therefore, targeting the leukotriene pathway may offer a strategy to modulate inflammation and potentially improve the efficacy of immunotherapies in S\_III subtype cancers.
\\

\bottomrule
\end{longtable}
}

\noindent \textbf{Conclusion 12.16: }FMOD's Association with Extracellular Matrix Remodeling and Metastasis

{
\rowcolors{1}{white}{white}
\centering
\normalsize
\begin{longtable}{>{\raggedright\arraybackslash}m{0.15\textwidth} >{\raggedright\arraybackslash}m{0.8\textwidth}}
\toprule

\textbf{Hypothesis} & 
The upregulation of FMOD in the S\_III subtype underscores its involvement in extracellular matrix remodeling, a key process in cancer metastasis. This suggests that interventions aimed at inhibiting FMOD could prevent tumor spread, especially in subtypes where its expression correlates with poor prognosis.
\\

\bottomrule
\end{longtable}
}

\noindent \textbf{Conclusion 12.17: }Unique Metabolic Dependencies in the S\_III Subtype

{
\rowcolors{1}{white}{white}
\centering
\normalsize
\begin{longtable}{>{\raggedright\arraybackslash}m{0.15\textwidth} >{\raggedright\arraybackslash}m{0.8\textwidth}}
\toprule

\textbf{Hypothesis} & 
The downregulation of pathways involved in bile acid and xenobiotic metabolism (CYP8B1, ETNK2) in the S\_III subtype hints at unique metabolic dependencies that could be exploited therapeutically. Targeting these metabolic pathways might selectively impact tumor cells' survival and proliferation in this subtype.
\\

\bottomrule
\end{longtable}
}

\noindent \textbf{Conclusion 12.18: }Differential Protein Expression and Implications for Personalized Medicine

{
\rowcolors{1}{white}{white}
\centering
\normalsize
\begin{longtable}{>{\raggedright\arraybackslash}m{0.15\textwidth} >{\raggedright\arraybackslash}m{0.8\textwidth}}
\toprule

\textbf{Hypothesis} & 
The differential expression of proteins such as RAB31, ALOX5AP, and FMOD, along with the distinct metabolic and inflammatory pathways enriched in the S\_III subtype, pave the way for personalized medicine approaches. By targeting these specific molecular alterations, therapies can be tailored to the unique proteomic landscape of the S\_III subtype, potentially improving treatment outcomes.
\\

\bottomrule
\end{longtable}
}

\noindent \textbf{Conclusion 12.19: }Bile Acid Metabolism and Xenobiotic Metabolism Pathways

{
\rowcolors{1}{white}{white}
\centering
\normalsize
\begin{longtable}{>{\raggedright\arraybackslash}m{0.15\textwidth} >{\raggedright\arraybackslash}m{0.8\textwidth}}
\toprule

\textbf{Hypothesis} & 
Bile acid metabolism and Xenobiotic metabolism pathways being highlighted in the ORA results suggest alterations in metabolic processes in the S\_III subtype. Metabolic reprogramming is a hallmark of cancer, affecting tumor growth, survival, and the response to treatment.
\\

\bottomrule
\end{longtable}
}

\noindent \textbf{Conclusion 12.20: }Allograft Rejection and IFN-gamma Response Pathways

{
\rowcolors{1}{white}{white}
\centering
\normalsize
\begin{longtable}{>{\raggedright\arraybackslash}m{0.15\textwidth} >{\raggedright\arraybackslash}m{0.8\textwidth}}
\toprule

\textbf{Hypothesis} & 
Allograft rejection and IFN-gamma response pathways are enriched, implying a strong immune response component in the S\_III subtype. This could suggest a more inflamed tumor microenvironment, which has implications for immunotherapy responsiveness.
\\

\bottomrule
\end{longtable}
}
